# Supplementary material for: AR-sieve Bootstrap for High-dimensional Time Series
Source: arXiv:2112.00414 source file (2025-12-08)
Supplement: Supplementary file 1 [file Supplemental_Sieve_bootstrap_HDTS_BSYZ.pdf]

## Supplement to “AR-sieve Bootstrap for High-dimensional Time Series”

Danling Bi 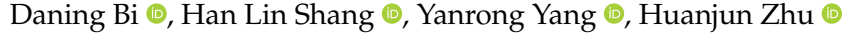, Han Lin Shang 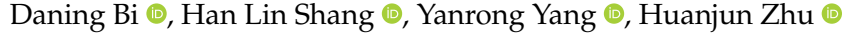, Yanrong Yang 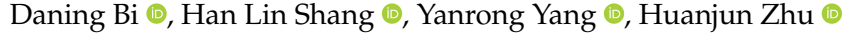, Huanjun Zhu 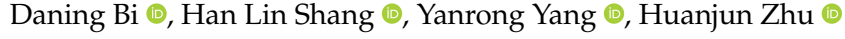

This supplementary material contains discussions of applying the proposed AR-sieve bootstrap on sparsely-observed functional time series, and technical proofs of results in the original paper “AR-sieve Bootstrap for High-dimensional Time Series”. In Appendix A, we introduce the smoothing problem on sparsely-observed functional time series and then propose to treating it as high-dimensional data when applying the AR-sieve bootstrap. Some simulations are also provided. In Appendix B, proofs of main theorems are presented, while some auxiliary lemmas and their proofs are left in Appendix C.

### A Applications on Sparsely-observed Functional Time Series

The second contribution of this work is that we compare the proposed novel AR-sieve bootstrap for high-dimensional time series with the AR-sieve bootstrap method for functional time series (Paparoditis 2018) in terms of their applications on sparse and unsmoothed functional observations. And we suggest that the sparse and unsmoothed observations need to be treated as high-dimensional time series and the AR-sieve bootstrap proposed in this work needs to be applied. In the literature of functional time series studies, a very fundamental assumption is that the actual observations come from a smoothed functional curve and statistical inferences for functional data usually require the observations to be dense. In a classic functional set-up, dense and discrete points are observed on a sample of  $T$  curves. Denoted by  $N_t$  the number of observations for the curve  $t$ , the discussions on the density of observations in functional data literature are generally through assumptions made on  $N_t$ . Typically, when  $N_t$  is much larger than the sample size  $T$ , the data can be considered dense functional data where each curve can be well smoothed before analysis. However, in the case where  $N_t$  is small compared with sample size  $T$  for all  $t$ , the discrete observations should be considered as sparse along the population functional curve. The fundamental problem of sparse functional data is that the local patterns of population functional curve are generally not captured by those sparse observations.

To illustrate the potential problems of pre-smoothing sparse observations for functional time series analysis, we consider a toy example. For a square-integrable functional process  $\{\mathcal{X}(u), u \in \mathcal{I}\}$ , let  $y_{i,t}$  be the  $i^{\text{th}}$  observation of  $\{\mathcal{X}_t(\cdot)\}$ , observed at a random time  $t$  with the measurement errors defined as  $\epsilon_{i,t}$  for  $t = 1, 2, \dots, T$  and  $i = 1, 2, \dots, N$ . Consider now for a model

of functional observations

$$y_{i,t} = \mathcal{X}_t(u_i) + \epsilon_{i,t}, \quad u_i \in \mathcal{I}, \quad (9)$$

where  $\epsilon_{i,t}$  is independent and identically distributed (i.i.d.) with  $\mathbb{E}(\epsilon_{i,t}) = 0$ ,  $\mathbb{V}(\epsilon_{i,t}) = \sigma^2$  and  $\mathcal{I}$  is a functional support. In this model, the observations of  $\{\mathcal{X}_t(\cdot)\}$  are assumed to be equally spaced, and the number of measurements  $N$  assesses the density and design of the actual observations. In the functional data analysis,  $\mathcal{X}_t(u_i)$  can be estimated or recovered by some smoothing methods such as a linear smoother as follows,

$$\widehat{\mathcal{X}}_t(u_i) = \sum_{j=1}^N w_i(u_j) y_{t,j},$$

where  $w_i(u_j)$  is the weight of  $j^{\text{th}}$  point on the  $i^{\text{th}}$  point with  $\sum_{j=1}^N w_i(u_j) = 1$  for  $t = 1, 2, \dots, T$  and  $i = 1, 2, \dots, N$ . The accuracy of the smoothing curve is highly related to the density of observations and measurement errors. If observations along the curve are equally spaced, the change of density can affect the quality of smoothness and its recovering power to the population curve. For a relatively sparse curve, smoothing can fail to work under certain situations; for example, when there are local patterns that observations are too sparse to capture. To visually depict this phenomenon, we provide a toy example by simulations in the following part. We consider a contaminated functional time series model generated from three Fourier bases with different frequencies reflecting local patterns. The details of the simulation setting can be found in Section A.1. The curves in Figure 5 are plotted based on 401 grid points defined on a functional support  $[0, 1]$ , whereas the actual number of observations  $N$  along each curve are chosen as 51, 21 and 5 to address different observation densities. As shown in Figure 5, when the observations (red points) become sparse (but still equally spaced), the (red) smoothing curve can lead to an obvious misleading result with local patterns not accurately captured by the smoothing curve. The errors associated with pre-smoothing on those sparse observations are generally large. In this situation, the assumption of dense functional data suffers from insufficient observations along each curve. As a result, we cannot adopt the pre-smoothing results based on functional set-up but instead treat the data as multivariate time series with growing dimensions. In other words, when  $N$  grows with sample size  $T$  but at a relatively slower rate, the real data may adapt to a high-dimensional set-up rather than a functional set-up, which makes statistical inferences and applications rather different. This phenomenon is associated with an area where functional data analysis and high-dimensional data analysis

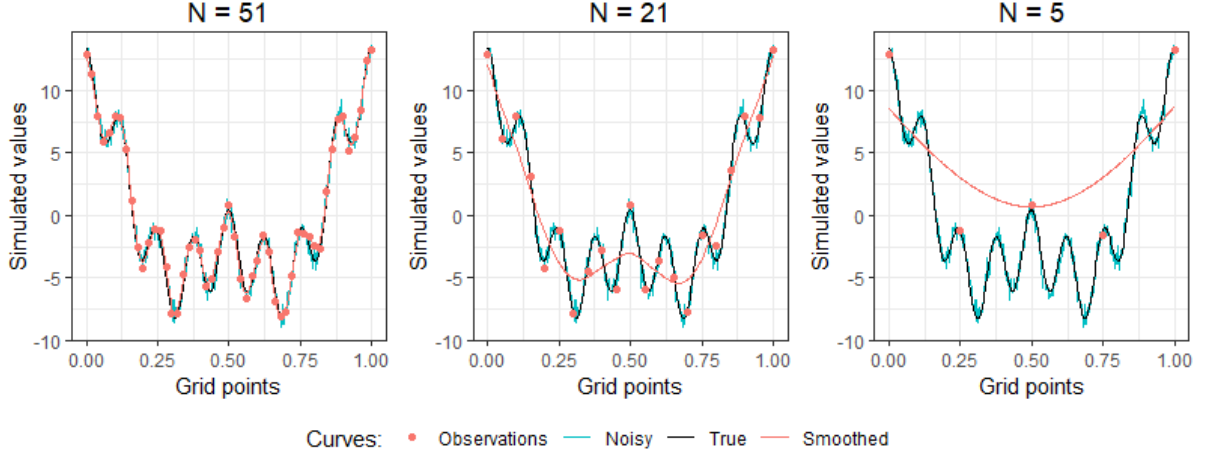

**Figure 5** Example of smoothing error of sparse functional time series observations

may overlap yet follow different assumptions and produce quite different asymptotic results.

In contrast to functional data analysis, where the increase of observations along a curve can practically improve pre-smoothing and recovering the functional curve, the growing of dimensions is associated with the increase of complexity for high-dimensional data analysis. This key difference makes it vital to choose between functional time series and high-dimensional time series methods. In the following part, we consider the situation where  $N$  is growing but not fast enough. The curve smoothed from the sparse observations is inaccurate, especially to local patterns of a functional curve. We apply the proposed AR-sieve bootstrap method for studying the inferences of this type of high-dimensional time series.

### A.1 Smoothing on sparse discrete functional time series

To study the impact of smoothing on the sparse functional time series observations, we can compare bootstrap samples' empirical distributions under various densities of observations. To start, we first assume the data are originated from functional curves, which are temporal dependent. Recall model (9) that

$$y_{t,i} = \mathcal{X}_t(u_i) + \epsilon_{t,i}, \quad u_i \in \mathcal{I},$$

where  $\epsilon_{t,i}$  is i.i.d. with  $\mathbb{E}(\epsilon_{t,i}) = 0$  and  $\mathbb{V}(\epsilon_{t,i}) = \sigma^2$ , for  $t = 1, 2, \dots, T$  and  $i = 1, 2, \dots, N$ . In this model, the number of measurements  $N$  reflect the density of the actual observations. To study the impact of density, we assume the observations are equally spaced and generated from a

three factors' model

$$\mathbf{y}_t = \mathbf{Q}\mathbf{f}_t + \mathbf{u}_t,$$

where  $u_{t,i}$ , the element in  $\{\mathbf{u}_t\}$ , is independent  $\mathcal{N}(0, 1)$  random noise,  $\mathbf{Q}$  is a  $N \times 3$  matrix with each column a Fourier basis and  $\cos(2\pi i/N)$ ,  $\cos(4\pi i/N)$ ,  $0.5 \cos(16\pi i/N)$  as  $i^{\text{th}}$  element, respectively. The factors  $\{\mathbf{f}_t\}$  follows a VAR(1) model with a coefficient matrix

$$\begin{bmatrix} 0.5 & 0.1 & 0.1 \\ 0.1 & 0.5 & 0.1 \\ 0.1 & 0.1 & 0.5 \end{bmatrix}$$

and errors independent simulated from  $\mathcal{N}(0, 1)$ . The Fourier basis is selected to produce a smoothed population curve, with the third basis reflecting local patterns. Hence, we can generate discrete observations from a functional curve with local patterns. In Section 1, we have presented plots of  $\{\mathbf{y}_t\}$  at a particular time  $t$  with three different densities of observations to illustrate a smoothing's potential issue. This section takes it one step further and considers a wider choice of densities so that the actual dimensions of observations along each curve are  $N = 101, 51, 21, 17, 11$  and  $5$ .

For the same choice of time  $t$  as in Section 1, we have generated 6 plots under various densities in Figure 6 to compare the smoothing results with the population true curve and noisy curve with small measurement errors. The smoothing results are obtained using B-splines with the number of basis functions set to  $N$ , the actual number of observations in each case, and the roughness penalties selected based on generalised cross-validation (GCV). As depicted in Figure 6, when the actual number of observations  $N$  is relatively small, for example,  $N < 21$ , some local patterns of the population curve are generally not captured. In addition, the smoothing curve sometimes also averaged out the actual observations to achieve relatively flat results, for example, when  $N = 21, 17$  and  $5$  as in Figure 6. As a result, the observations after smoothing are generally less spread than the original observations, which produces very different bootstrap samples and inferences' results. To see that, we generate  $B = 499$  AR-sieve bootstrap samples and computed two summary statistics to compare the bootstrap distribution based on original observations with smoothed observations. We use AR-sieve bootstrap to obtain estimates of a so-called (standardised) mean statistic, computed as  $\bar{y}^* = \frac{\sqrt{T}}{\sqrt{N}} \mathbf{1}^\top \hat{\mathbf{Q}} \mathbf{f}^*$  according to Theorem 4.2, and  $\delta_1^*$ , the estimate of (standardised) largest eigenvalue of symmetrised lag-1 sample autocovariance matrix as defined in Proposition 4.4, to compare bootstrap samples from original

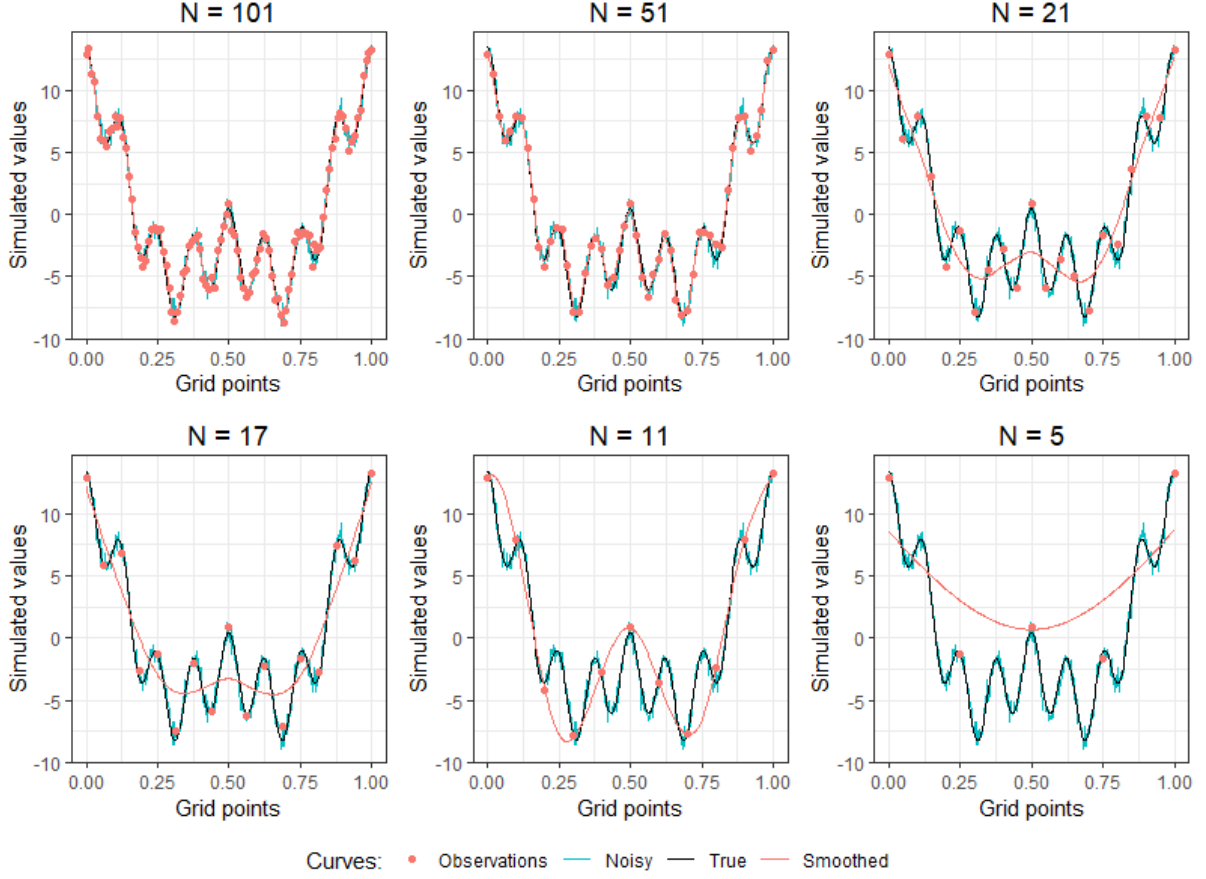

**Figure 6** Example of smoothing errors on sparse functional observations

observations with bootstrap samples from pre-smoothed observations.

Figures 7 and 8 compare the histograms and boxplots of  $\delta_1^*$ , the AR-sieve bootstrap estimates of largest eigenvalue of symmetrised lag-1 autocovariance matrix, while Figures 9 and 10 compare the histograms and boxplots of  $\overline{y}^*$ , the AR-sieve bootstrap estimates of the (standardised) mean statistic. As seen in Figure 6, when  $N = 21, 17$  and  $5$ , the pre-smoothed observations are averaged out compared with the original observations. As a result, the bootstrap estimates of the two statistics perform differently before and after smoothing, when  $N = 21, 17$  and  $5$ . Figures 7 and 9 use boxplots to present the difference of empirical distributions of  $\overline{y}^*$  and  $\delta_1^*$  for  $N = 21, 17$  and  $5$ , whereas Figures 8 and 10 illustrate the impact of smoothing by comparing the histograms of  $\overline{y}^*$  and  $\delta_1^*$ .

The last example we presented in Figure 11 illustrates results of AR-sieve bootstrap estimates (bootstrap average) of the functional mean curve when we pre-smooth the observations under various densities of data. As shown in Figure 11, when the actual observations are relatively dense, for example,  $N \geq 51$ , AR-sieve bootstrap estimates of the mean functional curve are close to the pre-smoothed curve and the population curve. However, when the observations are

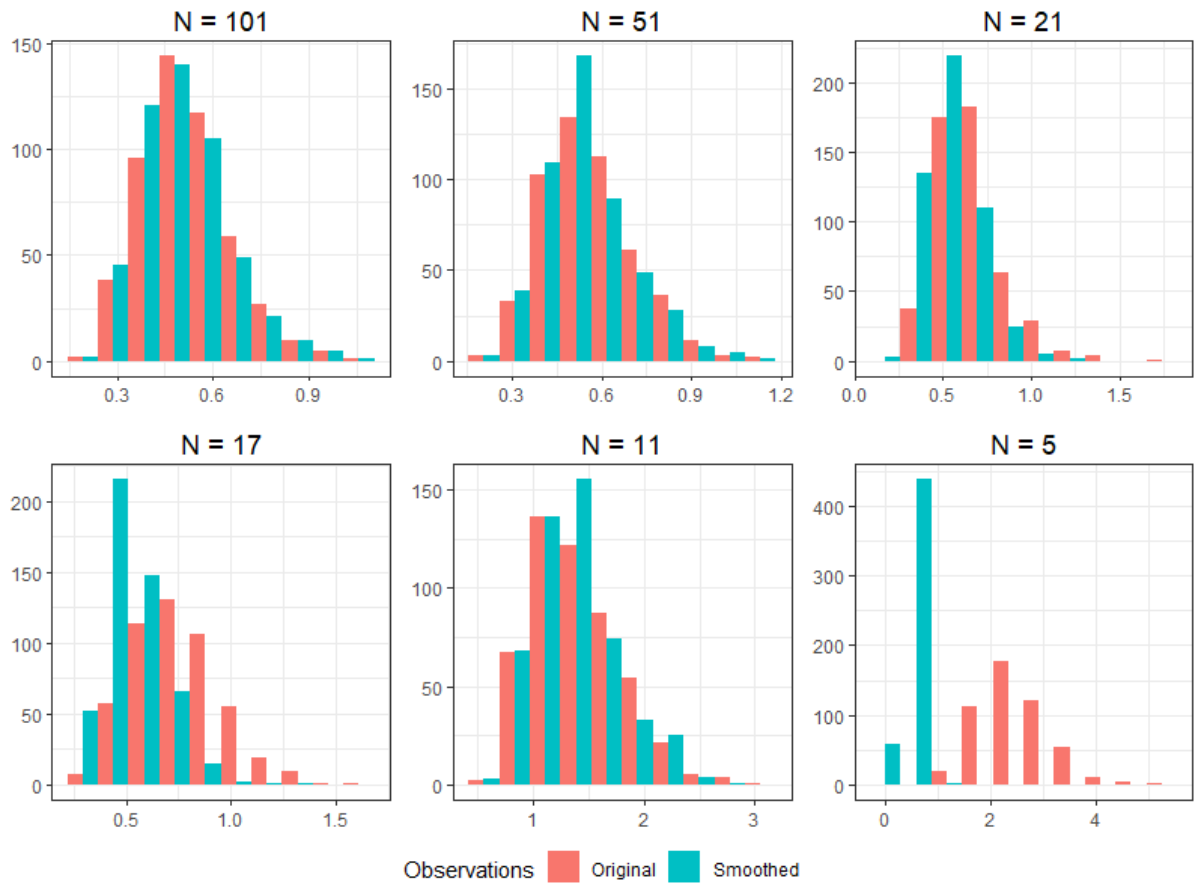

**Figure 7** Histograms of  $\delta_1^*$ , the AR-sieve bootstrap estimates of the largest eigenvalue of symmetrised lag-1 sample autocovariance matrix

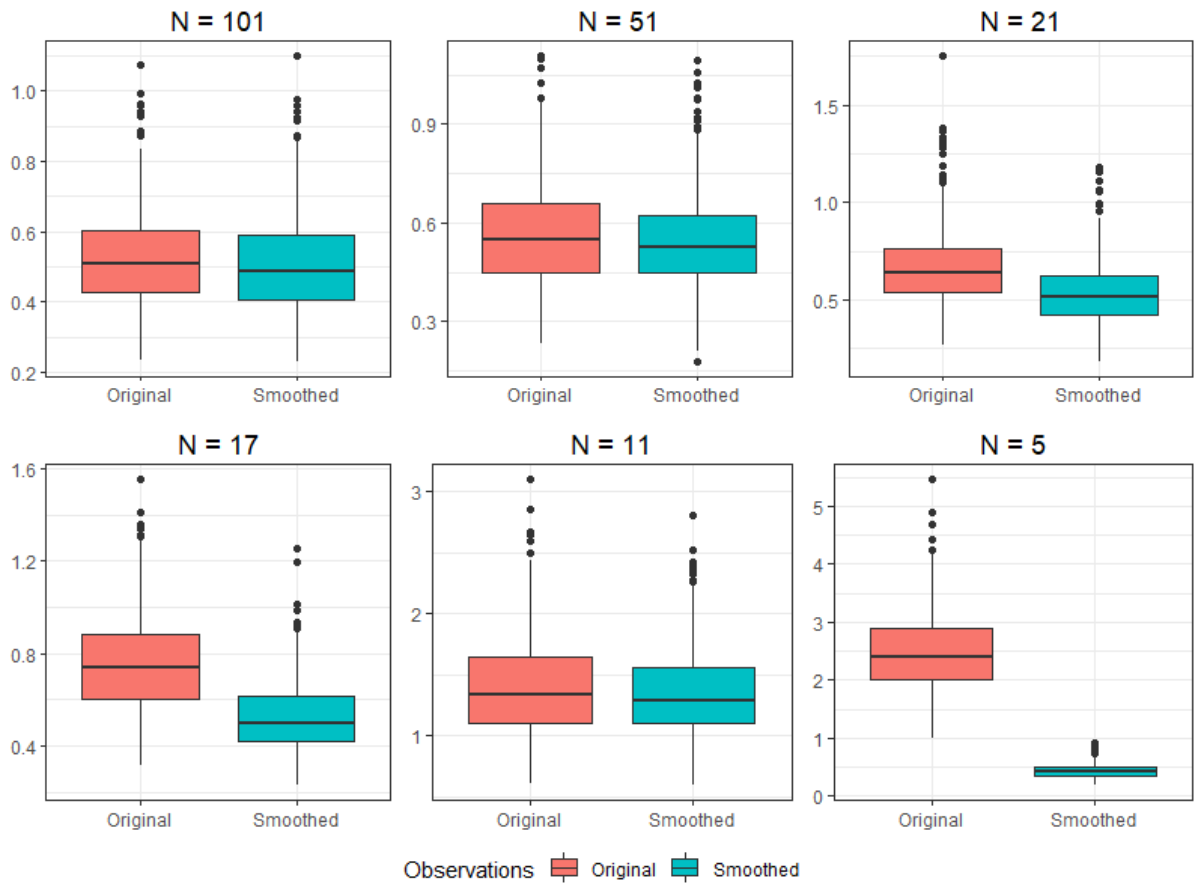

**Figure 8** Boxplots of  $\delta_1^*$ , the AR-sieve bootstrap estimates of the largest eigenvalue of symmetrised lag-1 sample autocovariance matrix

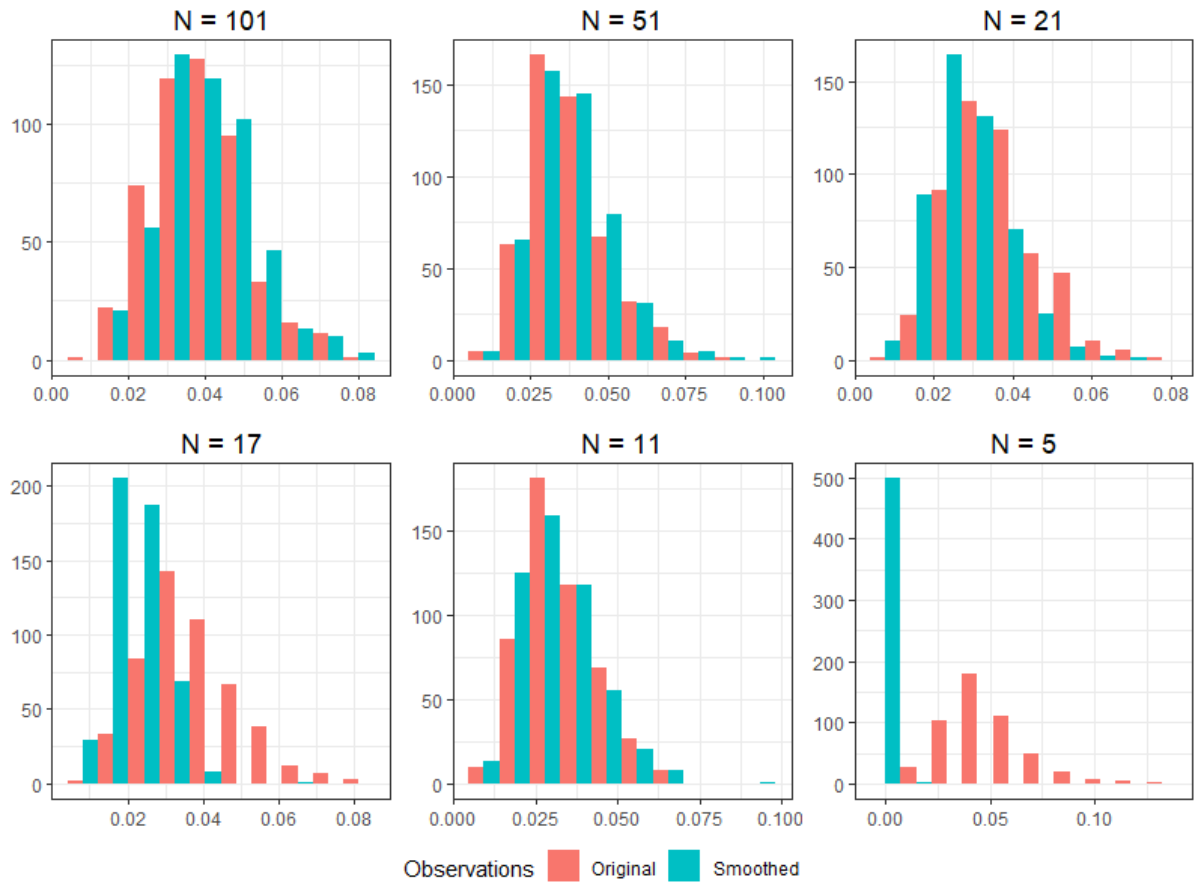

**Figure 9** Histograms of  $\overline{y^*}$ , the AR-sieve bootstrap estimates of the mean statistic



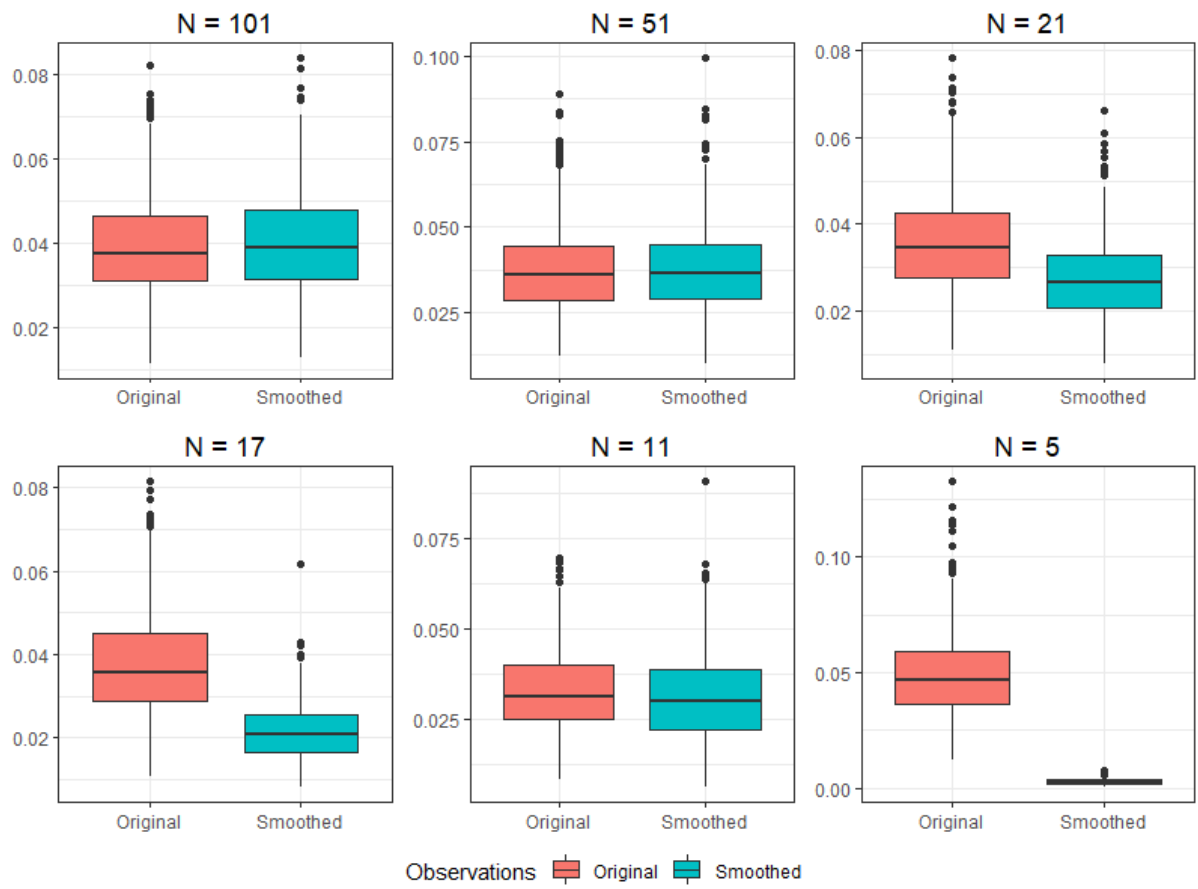

**Figure 10** Boxplots of  $\overline{\overline{y^*}}$ , the AR-sieve bootstrap estimates of the mean statistic

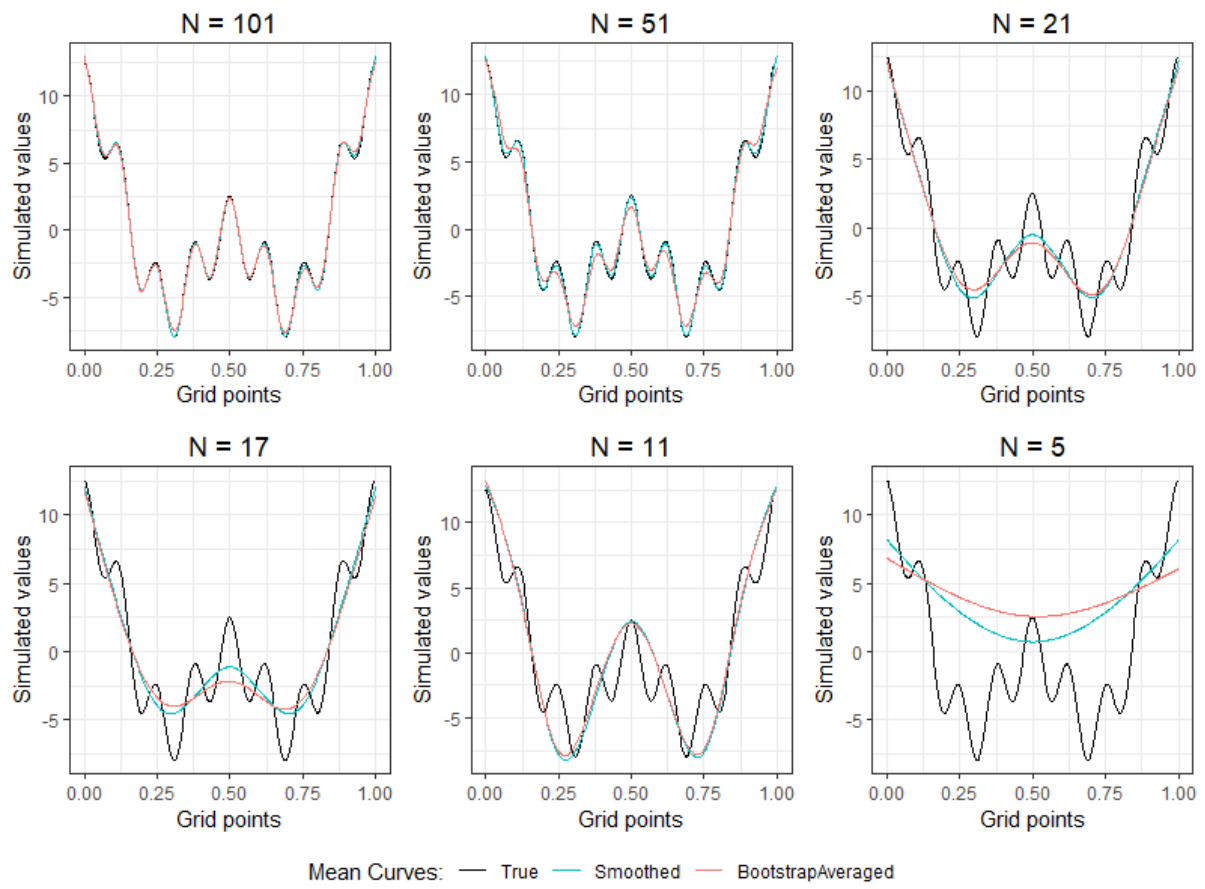

**Figure 11** Example of errors of the AR-sieve bootstrap mean curve for sparse functional observations

sparse, for example,  $N \leq 21$ , AR-sieve bootstrap estimates of the mean functional curve do not correctly capture the local patterns of the population curve, which is due to the unacceptable smoothing results. This result is also typical evidence of the impact of pre-smoothing on AR-sieve bootstrap for functional time series. Hence, when the actual functional time series observations are sparse, pre-smoothing may significantly impact statistical inferences, including bootstrap. In fact, for many real-world time series data, the rule on considering a data set as dense functional time series is generally not clear and often varies across researchers and problems. Practically speaking, the impact of observations' density is only about whether to pre-smooth the functional time series before performing bootstrap or other statistical analysis.

Nonetheless, the theoretical assumptions behind functional time series and high-dimensional time series vary, leading to very different theoretical results on statistical inferences, including AR-sieve bootstrap. On the other hand, this difference in data structure assumptions demonstrates the importance of developing statistical methods on sparse functional time series observations. It verifies our contributions on the building blocks of AR-sieve bootstrap for high-dimensional time series.

## B Technical proof of theorems

*Proof of Theorem 4.2.* Let  $\mathbf{f}_t^b = \sum_{l=1}^p \tilde{\mathbf{A}}_{l,p} \mathbf{f}_{t-l}^b + \mathbf{e}_{t,p}^b$ , where  $\{\tilde{\mathbf{A}}_{l,p}, l = 1, 2, \dots, p\}$  are the estimators of AR coefficient matrices based on true factors  $\{\mathbf{f}_t\}$ , and  $\{\mathbf{e}_{t,p}^b, t = p+1, p+2, \dots, T\}$  are generated by i.i.d. resampling from the centered residuals  $(\tilde{\mathbf{e}}_{t,p} - \bar{\tilde{\mathbf{e}}}_{T,p})$  with  $\tilde{\mathbf{e}}_{t,p} = \mathbf{f}_t - \sum_{l=1}^p \tilde{\mathbf{A}}_{l,p} \mathbf{f}_{t-l}$  and  $\bar{\tilde{\mathbf{e}}}_{T,p} = \frac{1}{T-p} \sum_{t=p+1}^T \tilde{\mathbf{e}}_{t,p}$ . Therefore,  $\{\mathbf{f}_t^b\}$  are bootstrap pseudo-variables generated based on the true factors  $\{\mathbf{f}_t\}$  rather than  $\{\hat{\mathbf{f}}_t\}$ . Recall that  $\{\mathbf{f}_t^*\}$  are bootstrapped based on the centered residuals  $(\hat{\mathbf{e}}_{t,p} - \bar{\hat{\mathbf{e}}}_{T,p})$  with  $\hat{\mathbf{e}}_{t,p} = \hat{\mathbf{f}}_t - \sum_{l=1}^p \hat{\mathbf{A}}_{l,p} \hat{\mathbf{f}}_{t-l}$  and  $\bar{\hat{\mathbf{e}}}_{T,p} = \frac{1}{T-p} \sum_{t=p+1}^T \hat{\mathbf{e}}_{t,p}$ , and we define  $\mathbb{E}^*$  and  $\text{Cov}^*$  as the expectation and covariance with respect to the measure assigning probability  $1/(T-p)$  to each observation, respectively. Therefore,  $\mathbb{E}^* \bar{\mathbf{f}}_T^* = \bar{\hat{\mathbf{f}}}_T$  by definition and we can write

$$\begin{aligned} \sqrt{T} \mathbf{c}^\top \hat{\mathbf{Q}} (\bar{\mathbf{f}}_T^* - \mathbb{E}^* \bar{\mathbf{f}}_T^*) &=: \mathcal{M}_1 + \mathcal{M}_2 + \mathcal{M}_3 \\ &= \sqrt{T} \mathbf{c}^\top \mathbf{Q} (\bar{\mathbf{f}}_T^b - \mathbb{E}^* \bar{\mathbf{f}}_T^b) + \sqrt{T} \mathbf{c}^\top (\hat{\mathbf{Q}} - \mathbf{Q}) (\bar{\mathbf{f}}_T^* - \mathbb{E}^* \bar{\mathbf{f}}_T^*) \\ &\quad + \sqrt{T} \mathbf{c}^\top \mathbf{Q} \left[ (\bar{\mathbf{f}}_T^* - \mathbb{E}^* \bar{\mathbf{f}}_T^*) - (\bar{\mathbf{f}}_T^b - \mathbb{E}^* \bar{\mathbf{f}}_T^b) \right], \end{aligned}$$

with obvious definitions of  $\mathcal{M}_1, \mathcal{M}_2$  and  $\mathcal{M}_3$ .

For the term  $\mathcal{M}_1$ , under Assumptions 3.1 (iii), 4.1 and the additional assumption in Theorem

4.2 that  $\lim_{T \rightarrow \infty} \mathbb{V}(\sqrt{T}\bar{\mathbf{f}}_T) = \sum_{k \in \mathbb{Z}} \Gamma_{\mathbf{f}}(k) < \infty$ , using Theorem 2.1 in Politis et al. (1997), we have the following CLT for  $\sqrt{T}\bar{\mathbf{f}}_T$

$$\sqrt{T}(\bar{\mathbf{f}}_T - \mathbb{E}\bar{\mathbf{f}}_T) \xrightarrow{d} \mathcal{N}\left(0, \sum_{k \in \mathbb{Z}} \Gamma_{\mathbf{f}}(k)\right).$$

Moreover, under the additional assumptions in Theorem 4.2,  $\mathbf{c}^\top \mathbf{Q}$  is an  $r$ -dimensional vector such that  $\|\mathbf{c}^\top \mathbf{Q}\|_{\ell_1} < \infty$  for a fixed  $r$ . Therefore, under Assumptions 3.1 (ii) and 4.1, we can use Cramer-Wold Theorem (Cramér & Wold 1936) to conclude for the scalar  $\sqrt{T}\mathbf{c}^\top \mathbf{Q}\bar{\mathbf{f}}_T$  that

$$\sqrt{T}\mathbf{c}^\top \mathbf{Q}(\bar{\mathbf{f}}_T - \mathbb{E}\bar{\mathbf{f}}_T) \xrightarrow{d} \mathcal{N}\left(0, \mathbf{c}^\top \mathbf{Q}\left(\sum_{k \in \mathbb{Z}} \Gamma_{\mathbf{f}}(k)\right)\mathbf{Q}^\top \mathbf{c}\right),$$

when  $T, N \rightarrow \infty$ .

Besides, under the strong mixing condition on true factors  $\{\mathbf{f}_t\}$ , the empirical moments of  $\{\mathbf{e}_t\}$  converge to its population counterpart. Therefore, under all the assumptions of 4.2, we fulfil all the conditions of Theorem 4.1 in Meyer & Kreiss (2015). Consequently, we can use Theorem 4.1 in Meyer & Kreiss (2015) to conclude that the general VAR-sieve bootstrap is valid for  $\sqrt{T}\mathbf{c}^\top \mathbf{Q}\bar{\mathbf{f}}_T$  since  $\sqrt{T}\mathbf{c}^\top \mathbf{Q}\bar{\mathbf{f}}_T$  shares the same CLT with its counterpart generated from the companion process as discussed in Meyer & Kreiss (2015). Hence

$$d_K\left(\mathcal{L}\left(\sqrt{T}\mathbf{c}^\top \hat{\mathbf{Q}}(\bar{\mathbf{f}}_T^* - \mathbb{E}^*\bar{\mathbf{f}}_T^*) \mid \mathbf{y}_1, \mathbf{y}_2, \dots, \mathbf{y}_T\right), \mathcal{L}\left(\sqrt{T}\mathbf{c}^\top \mathbf{Q}(\bar{\mathbf{f}}_T - \mathbb{E}\bar{\mathbf{f}}_T)\right)\right) = o_P(1)$$

as  $T, N \rightarrow \infty$ .

Therefore, to see the assertion in Theorem 4.2, we need to show that when  $T, N \rightarrow \infty$ , both  $\mathcal{M}_2$  and  $\mathcal{M}_3$  tend to 0 in probability, then apply Slutsky's theorem.

To show  $\mathcal{M}_2 \rightarrow 0$  in probability for  $T, N \rightarrow \infty$ , we first of all notice that

$$\sqrt{T}\mathbf{c}^\top (\hat{\mathbf{Q}} - \mathbf{Q})(\bar{\mathbf{f}}_T^* - \mathbb{E}^*\bar{\mathbf{f}}_T^*) = \frac{1}{\sqrt{T}}\mathbf{c}^\top (\hat{\mathbf{Q}} - \mathbf{Q}) \sum_{t=1}^T (\mathbf{f}_t^* - \bar{\mathbf{f}}_T).$$

Therefore, we can show that

$$\begin{aligned}
& \mathbb{E} \left[ \sqrt{T} \mathbf{c}^\top (\hat{\mathbf{Q}} - \mathbf{Q}) (\bar{\mathbf{f}}_T^* - \mathbb{E} \bar{\mathbf{f}}_T^*) \right]^2 \\
&= \mathbb{E} \left[ \frac{1}{T} \mathbf{c}^\top (\hat{\mathbf{Q}} - \mathbf{Q}) \sum_{t=1}^T (\mathbf{f}_t^* - \bar{\mathbf{f}}_T) \right] \left[ \sum_{s=1}^T (\mathbf{f}_s^* - \bar{\mathbf{f}}_T)^\top (\hat{\mathbf{Q}} - \mathbf{Q})^\top \mathbf{c} \right] \\
&= \left[ \frac{1}{T} \mathbf{c}^\top (\hat{\mathbf{Q}} - \mathbf{Q}) \sum_{t=1}^T \sum_{s=1}^T \mathbb{E} (\mathbf{f}_t^* - \bar{\mathbf{f}}_T) (\mathbf{f}_s^* - \bar{\mathbf{f}}_T)^\top (\hat{\mathbf{Q}} - \mathbf{Q})^\top \mathbf{c} \right] \\
&\leq \frac{1}{T} \left\| \mathbf{c}^\top (\hat{\mathbf{Q}} - \mathbf{Q}) \right\|^2 \left\| \sum_{t=1}^T \sum_{s=1}^T \mathbb{E} (\mathbf{f}_t^* - \bar{\mathbf{f}}_T) (\mathbf{f}_s^* - \bar{\mathbf{f}}_T)^\top \right\|_F \\
&= O_P \left( \frac{1}{T^2} \left\| \sum_{t=1}^T \sum_{s=1}^T \mathbb{E} (\mathbf{f}_t^* - \bar{\mathbf{f}}_T) (\mathbf{f}_s^* - \bar{\mathbf{f}}_T)^\top \right\|_F \right),
\end{aligned}$$

Define  $\Sigma_{e,p}^* := \mathbb{E}^* (\mathbf{e}_t^* \mathbf{e}_t^{*\top})$ , then

$$\begin{aligned}
\sum_{t=1}^T \sum_{s=1}^T \mathbb{E}^* (\mathbf{f}_t^* - \bar{\mathbf{f}}_T) (\mathbf{f}_s^* - \bar{\mathbf{f}}_T)^\top &= \sum_{t=1}^T \sum_{s=1}^T \mathbb{E}^* \left( \left( \sum_{l_1=0}^{\infty} \hat{\Psi}_{l_1,p} \mathbf{e}_{t-l_1}^* \right) \left( \sum_{l_2=0}^{\infty} \hat{\Psi}_{l_2,p} \mathbf{e}_{s-l_2}^* \right)^\top \right) \\
&= \sum_{t=1}^T \sum_{s=1}^T \mathbb{E}^* \sum_{l_1=0}^{\infty} \sum_{l_2=0}^{\infty} (\hat{\Psi}_{l_1,p} \mathbf{e}_{t-l_1}^* \mathbf{e}_{s-l_2}^{*\top} \hat{\Psi}_{l_2,p}^\top) \\
&= \sum_{t=1}^T \sum_{s=1}^T \sum_{l=0}^{\infty} \hat{\Psi}_{l,p} \mathbb{E}^* (\mathbf{e}_{t-l}^* \mathbf{e}_{s-l}^{*\top}) \hat{\Psi}_{s-t+l,p}^\top
\end{aligned}$$

where  $\mathbf{e}_{t-l_1}^*$  and  $\mathbf{e}_{s-l_2}^*$  are i.i.d. bootstrapped therefore  $\mathbb{E}^* (\mathbf{e}_{t-l_1}^* \mathbf{e}_{s-l_2}^{*\top}) = \mathbf{0}$  for  $l_1 \neq l_2$ .

Hence we can show that

$$\begin{aligned}
\frac{1}{T^2} \left\| \sum_{t=1}^T \sum_{s=1}^T \mathbb{E}^* (\mathbf{f}_t^* - \bar{\mathbf{f}}_T) (\mathbf{f}_s^* - \bar{\mathbf{f}}_T)^\top \right\|_F &\leq \frac{1}{T^2} \left\| \Sigma_{e,p}^* \right\|_F \sum_{l=0}^{\infty} \left\| \hat{\Psi}_{l,p} \right\|_F \sum_{t=1}^T \sum_{s=1}^T \left\| \hat{\Psi}_{s-t+l,p} \right\|_F \\
&= O_P \left( \frac{1}{T} \right),
\end{aligned}$$

where we note that Lemmas C.5 and C.7 imply the summability of  $\left\| \hat{\Psi}_{l,p} \right\|_F$ , hence  $\sum_{s=1}^T \left\| \hat{\Psi}_{s-t+l,p} \right\|_F$  is bounded for  $T \rightarrow \infty$ . Therefore,  $\frac{1}{T} \sum_{l=0}^{\infty} \left\| \hat{\Psi}_{l,p} \right\|_F \sum_{t=1}^T \sum_{s=1}^T \left\| \hat{\Psi}_{s-t+l,p} \right\|_F$  is bounded for  $T \rightarrow \infty$ , and we can conclude that  $\mathbb{E}^* \left[ \sqrt{T} \mathbf{c}^\top (\hat{\mathbf{Q}} - \mathbf{Q}) (\bar{\mathbf{f}}_T^* - \mathbb{E}^* \bar{\mathbf{f}}_T^*) \right]^2 \rightarrow 0$  in probability, which suffices for  $\mathcal{M}_2 \rightarrow 0$  in probability conditional on the sample.

For  $\mathcal{M}_3$ , we first write

$$\begin{aligned}
& \mathbb{E}^* \left[ \sqrt{T} \mathbf{c}^\top \mathbf{Q} \left\{ (\overline{\mathbf{f}_T^*} - \mathbb{E}^* \overline{\mathbf{f}_T^*}) - (\overline{\mathbf{f}_T^b} - \mathbb{E}^* \overline{\mathbf{f}_T^b}) \right\} \right]^2 \\
&= \mathbb{E}^* \left\| \sqrt{T} \mathbf{c}^\top \mathbf{Q} \left\{ (\overline{\mathbf{f}_T^*} - \widehat{\mathbf{f}_T}) - (\overline{\mathbf{f}_T^b} - \widetilde{\mathbf{f}_T}) \right\} \right\|^2 \\
&\leq \|\mathbf{c}^\top \mathbf{Q}\|^2 \frac{1}{T} \sum_{t=1}^T \sum_{s=1}^T \mathbb{E}^* \left\| \left\{ (\mathbf{f}_t^* - \widehat{\mathbf{f}_T}) - (\mathbf{f}_t^b - \widetilde{\mathbf{f}_T}) \right\} \left\{ (\mathbf{f}_s^* - \widehat{\mathbf{f}_T}) - (\mathbf{f}_s^b - \widetilde{\mathbf{f}_T}) \right\}^\top \right\|_F \\
&= O_p \left( \frac{1}{T} \sum_{t=1}^T \sum_{s=1}^T \mathbb{E}^* \left\| \left\{ (\mathbf{f}_t^* - \widehat{\mathbf{f}_T}) - (\mathbf{f}_t^b - \widetilde{\mathbf{f}_T}) \right\} \left\{ (\mathbf{f}_s^* - \widehat{\mathbf{f}_T}) - (\mathbf{f}_s^b - \widetilde{\mathbf{f}_T}) \right\}^\top \right\|_F \right),
\end{aligned}$$

where the last line follows from the fact that  $\|\mathbf{c}^\top \mathbf{Q}\|^2$  is bounded when  $N \rightarrow \infty$ . To proceed, first note that

$$\begin{aligned}
& \frac{1}{T} \sum_{t=1}^T \sum_{s=1}^T \mathbb{E}^* \left\{ \left( \mathbf{f}_t^* - \widehat{\mathbf{f}_T} \right) - \left( \mathbf{f}_t^b - \widetilde{\mathbf{f}_T} \right) \right\} \left\{ \left( \mathbf{f}_s^* - \widehat{\mathbf{f}_T} \right) - \left( \mathbf{f}_s^b - \widetilde{\mathbf{f}_T} \right) \right\}^\top \\
&= \frac{1}{T} \sum_{t=1}^T \sum_{s=1}^T \mathbb{E}^* \left\{ \sum_{l_1=0}^{\infty} \widehat{\Psi}_{l_1,p} \mathbf{e}_{t-l_1,p}^* - \widetilde{\Psi}_{l_1,p} \mathbf{e}_{t-l_1,p}^b \right\} \left\{ \sum_{l_2=0}^{\infty} \widehat{\Psi}_{l_2,p} \mathbf{e}_{s-l_2,p}^* - \widetilde{\Psi}_{l_2,p} \mathbf{e}_{s-l_2,p}^b \right\}^\top \\
&= \frac{1}{T} \sum_{t=1}^T \sum_{s=1}^T \mathbb{E}^* \left\{ \sum_{l_1=0}^{\infty} \widehat{\Psi}_{l_1,p} \mathbf{e}_{t-l_1,p}^* \right\} \left\{ \sum_{l_2=0}^{\infty} \widehat{\Psi}_{l_2,p} \mathbf{e}_{s-l_2,p}^* - \widetilde{\Psi}_{l_2,p} \mathbf{e}_{s-l_2,p}^b \right\}^\top \\
&\quad + \frac{1}{T} \sum_{t=1}^T \sum_{s=1}^T \mathbb{E}^* \left\{ \sum_{l_1=0}^{\infty} \widetilde{\Psi}_{l_1,p} \mathbf{e}_{t-l_1,p}^b \right\} \left\{ \sum_{l_2=0}^{\infty} \widetilde{\Psi}_{l_2,p} \mathbf{e}_{s-l_2,p}^b - \widehat{\Psi}_{l_2,p} \mathbf{e}_{s-l_2,p}^* \right\}^\top \\
&=: \frac{1}{T} \sum_{t=1}^T \sum_{s=1}^T (\mathcal{H}_1 + \mathcal{H}_2),
\end{aligned}$$

with an obvious notation for  $\mathcal{H}_1$  and  $\mathcal{H}_2$ . Then, we only consider  $\mathcal{H}_1$  as  $\mathcal{H}_2$  can be dealt with similarly.

For  $\mathcal{H}_1$ , we can further decompose it as

$$\begin{aligned}
\mathcal{H}_1 &= \sum_{s=1}^T \mathbb{E}^* \left\{ \sum_{l_1=0}^{\infty} \widehat{\Psi}_{l_1,p} \mathbf{e}_{t-l_1,p}^* \right\} \left\{ \sum_{l_2=0}^{\infty} \widehat{\Psi}_{l_2,p} \mathbf{e}_{s-l_2,p}^* - \widetilde{\Psi}_{l_2,p} \mathbf{e}_{s-l_2,p}^b \right\}^\top \\
&\quad + \sum_{s=1}^T \mathbb{E}^* \left\{ \sum_{l_1=0}^{\infty} \widehat{\Psi}_{l_1,p} \mathbf{e}_{t-l_1,p}^* \right\} \left\{ \sum_{l_2=0}^{\infty} \widetilde{\Psi}_{l_2,p} \mathbf{e}_{s-l_2,p}^* - \widetilde{\Psi}_{l_2,p} \mathbf{e}_{s-l_2,p}^b \right\}^\top \\
&= \sum_{s=1}^T \sum_{l=0}^{\infty} \widehat{\Psi}_{l,p} \mathbb{E}^* \left\{ \mathbf{e}_{t-l,p}^* \mathbf{e}_{t-l,p}^{*\top} \right\} \left\{ \widehat{\Psi}_{l+s-t,p} - \widetilde{\Psi}_{l+s-t,p} \right\}^\top \\
&\quad + \sum_{s=1}^T \sum_{l=0}^{\infty} \widehat{\Psi}_{l,p} \mathbb{E}^* \left\{ \mathbf{e}_{t-l,p}^* (\mathbf{e}_{t-l,p}^* - \mathbf{e}_{t-l,p}^b)^\top \right\} \widetilde{\Psi}_{l+s-t,p}^\top \\
&=: \mathcal{H}_{11} + \mathcal{H}_{12}.
\end{aligned}$$

where the second last line follows from the bootstrap independence for  $l_1 \neq l_2$ . Hence we can conclude for  $\mathcal{H}_{11}$  that

$$\begin{aligned}
\frac{1}{T} \sum_{t=1}^T \sum_{s=1}^T \|\mathcal{H}_{11}\|_F &= \frac{1}{T} \sum_{t=1}^T \sum_{s=1}^T \left\| \sum_{l=0}^{\infty} \hat{\Psi}_{l,p} \Sigma_{e,p}^* \left\{ \hat{\Psi}_{l+s-t,p} - \tilde{\Psi}_{l+s-t,p} \right\}^\top \right\|_F \\
&\leq \left\| \Sigma_{e,p}^* \right\|_F \frac{1}{T} \sum_{l=0}^{\infty} \left\| \hat{\Psi}_{l,p} \right\|_F \sum_{t=1}^T \sum_{s=1}^T \left\| \hat{\Psi}_{l+s-t,p} - \tilde{\Psi}_{l+s-t,p} \right\|_F \\
&= O_P \left( p^{\frac{3}{2}} \left\| \hat{\mathbf{A}}_p - \tilde{\mathbf{A}}_p \right\|_F \right) \\
&= o_P(1),
\end{aligned}$$

where the second last line follows from the results in Lemmas C.5 and C.7, and the last line follows the result in Lemma C.7.

For  $\mathcal{H}_{12}$  we can show that

$$\begin{aligned}
\frac{1}{T} \sum_{t=1}^T \sum_{s=1}^T \|\mathcal{H}_{12}\|_F &\leq \sqrt{\mathbb{E}^* \left\| e_{t,p}^* \right\|^2} \sqrt{\mathbb{E}^* \left\| e_{t,p}^* - e_{t,p}^b \right\|^2} \frac{1}{T} \sum_{l=0}^{\infty} \left\| \hat{\Psi}_{l,p} \right\|_F \sum_{t=1}^T \sum_{s=1}^T \left\| \hat{\Psi}_{l+s-t,p} \right\|_F \\
&= O_P \left( \sqrt{\mathbb{E}^* \left\| e_{t,p}^* - e_{t,p}^b \right\|^2} \right),
\end{aligned}$$

where the last line follows from the same arguments on summability properties in Lemmas C.5. Hence it remains to show  $\mathbb{E}^* \left\| e_{t,p}^* - e_{t,p}^b \right\|^2 \rightarrow 0$  in probability. Recall that  $\mathbb{E}^*$  defines expectation with respect to the measure assigning probability  $1/(T-p)$  to each observation, this follows as

$$\begin{aligned}
\mathbb{E}^* \left\| e_{t,p}^* - e_{t,p}^b \right\|^2 &= \mathbb{E}^* \left\{ \left( e_{t,p}^* - e_{t,p}^b \right) \left( e_{t,p}^* - e_{t,p}^b \right)^\top \right\} \\
&= \frac{1}{T-p} \sum_{t=p+1}^T \left\{ \left( \hat{e}_{t,p} - \bar{\tilde{e}}_{T,p} \right) - \left( \tilde{e}_{t,p} - \bar{\tilde{e}}_{T,p} \right) \right\} \left\{ \left( \hat{e}_{t,p} - \bar{\tilde{e}}_{T,p} \right) - \left( \tilde{e}_{t,p} - \bar{\tilde{e}}_{T,p} \right) \right\}^\top \\
&= \frac{1}{T-p} \sum_{t=p+1}^T \left\{ \left( \hat{e}_{t,p} - \tilde{e}_{t,p} \right) - \left( \bar{\tilde{e}}_{T,p} - \bar{\tilde{e}}_{T,p} \right) \right\} \left\{ \left( \hat{e}_{t,p} - \tilde{e}_{t,p} \right) - \left( \bar{\tilde{e}}_{T,p} - \bar{\tilde{e}}_{T,p} \right) \right\}^\top \\
&\leq \frac{2}{T-p} \sum_{t=p+1}^T \left\| \hat{e}_{t,p} - \tilde{e}_{t,p} \right\|^2 + 2 \left\{ \left\| \bar{\tilde{e}}_{T,p} \right\|^2 + \left\| \bar{\tilde{e}}_{T,p} \right\|^2 - 2 \left\| \bar{\tilde{e}}_{T,p} \right\| \left\| \bar{\tilde{e}}_{T,p} \right\| \right\} \\
&\leq \frac{2}{T-p} \sum_{t=p+1}^T \left\| \hat{e}_{t,p} - \tilde{e}_{t,p} \right\|^2 + 4 \left\{ \left\| \bar{\tilde{e}}_{T,p} \right\|^2 + \left\| \bar{\tilde{e}}_{T,p} \right\|^2 \right\}.
\end{aligned}$$

Recall that when  $\{\mathbf{f}_t\}$  and  $\{\hat{\mathbf{f}}_t\}$  have non-zero means,  $\tilde{e}_{t,p} = (\mathbf{f}_t - \bar{\mathbf{f}}_T) - \sum_{l=1}^p \tilde{\mathbf{A}}_{l,p} (\mathbf{f}_{t-l} - \bar{\mathbf{f}}_T)$  and  $\hat{e}_{t,p} = (\hat{\mathbf{f}}_t - \bar{\hat{\mathbf{f}}}_T) - \sum_{l=1}^p \hat{\mathbf{A}}_{l,p} (\hat{\mathbf{f}}_{t-l} - \bar{\hat{\mathbf{f}}}_T)$ . Without altering the idea of proof, to simplify the notations used, we use  $\{\mathbf{f}_t\}$  and  $\{\hat{\mathbf{f}}_t\}$  to denote the demeaned factors  $(\mathbf{f}_t - \bar{\mathbf{f}}_T)$  and their sample counterparts  $(\hat{\mathbf{f}}_t - \bar{\hat{\mathbf{f}}}_T)$ , respectively. Therefore, with the same arguments in the proof

of Lemma C.8, we have

$$\begin{aligned}
\frac{2}{T-p} \sum_{t=p+1}^T \|\hat{e}_{t,p} - \tilde{e}_{t,p}\|^2 &= \frac{2}{T-p} \sum_{t=p+1}^T \left\| (\hat{\mathbf{f}}_t - \mathbf{f}_t) + \sum_{l=1}^p (\tilde{\mathbf{A}}_{l,p} \mathbf{f}_{t-l} - \hat{\mathbf{A}}_{l,p} \hat{\mathbf{f}}_{t-l}) \right\|^2 \\
&\leq \frac{4}{T-p} \sum_{t=p+1}^T \|\hat{\mathbf{f}}_t - \mathbf{f}_t\|^2 + \frac{4}{T-p} \sum_{t=p+1}^T \left\| \sum_{l=1}^p \tilde{\mathbf{A}}_{l,p} \mathbf{f}_{t-l} - \hat{\mathbf{A}}_{l,p} \hat{\mathbf{f}}_{t-l} \right\|^2 \\
&\leq \frac{4}{T-p} \sum_{t=p+1}^T \|\hat{\mathbf{f}}_t - \mathbf{f}_t\|^2 + 8 \sum_{l=1}^p \|\hat{\mathbf{A}}_{l,p}\|_F^2 \frac{1}{T-p} \sum_{t=p+1}^T \|\hat{\mathbf{f}}_{t-l} - \mathbf{f}_{t-l}\|^2 \\
&\quad + 8 \left\| \sum_{l=1}^p (\hat{\mathbf{A}}_{l,p} - \tilde{\mathbf{A}}_{l,p}) \frac{1}{T-p} \sum_{t=p+1}^T \mathbf{f}_{t-l} \right\|_F^2 \\
&= O_P \left( \sup_{p+1 \leq t \leq T} \|\hat{\mathbf{f}}_t - \mathbf{f}_t\|^2 \right) + O_P \left( \left\| \sum_{l=1}^p (\hat{\mathbf{A}}_{l,p} - \tilde{\mathbf{A}}_{l,p}) \right\|_F^2 \right) \\
&= O_P \left( \left( \frac{1}{\sqrt{T}} + \frac{1}{\sqrt{N}} \right)^2 \right) + O_P \left( p^8 \left( \frac{1}{\sqrt{T}} + \frac{1}{\sqrt{N}} \right)^2 \right) \\
&= o_P(1), \tag{10}
\end{aligned}$$

where the third last line follows from the fact that  $\|\hat{\mathbf{A}}_{l,p}\|_F^2$  is summable, which is implied by Assumption 4.2 and Lemma C.3. The second last line is then a direct result of Lemmas C.3 and C.4, and Assumption 4.3 implies the last line.

Furthermore,  $\bar{\mathbf{e}}_{T,p} = \frac{1}{T-p} \sum_{t=p+1}^T \hat{\mathbf{e}}_{t,p} = \frac{1}{T-p} \sum_{t=p+1}^T \left( \hat{\mathbf{f}}_t - \sum_{l=1}^p \hat{\mathbf{A}}_{l,p} \hat{\mathbf{f}}_{t-l} \right)$  and we can show that

$$\|\bar{\mathbf{e}}_{T,p}\|^2 \leq 2 \left\| \frac{1}{T-p} \sum_{t=p+1}^T \hat{\mathbf{f}}_t \right\|^2 + 2 \left\| \sum_{l=1}^p \hat{\mathbf{A}}_{l,p} \frac{1}{T-p} \sum_{t=p+1}^T \hat{\mathbf{f}}_{t-l} \right\|^2 = o_P(1). \tag{11}$$

This is because, firstly

$$\begin{aligned}
\left\| \frac{1}{T-p} \sum_{t=p+1}^T \hat{\mathbf{f}}_t \right\|^2 &\leq 2 \left\| \frac{1}{T-p} \sum_{t=p+1}^T \mathbf{f}_t \right\|^2 + 2 \left\| \frac{1}{T-p} \sum_{t=p+1}^T (\hat{\mathbf{f}}_t - \mathbf{f}_t) \right\|^2 \\
&= O_P \left( \frac{1}{T-p} \right) + O_P \left( \frac{1}{T-p} \sum_{t=p+1}^T \|\hat{\mathbf{f}}_t - \mathbf{f}_t\|^2 \right) \\
&= O_P \left( \frac{1}{T-p} \right) + O_P \left( \left( \frac{1}{\sqrt{T}} + \frac{1}{\sqrt{N}} \right)^2 \right) = o_P(1),
\end{aligned}$$

where the second last line follows as we have assumed the population mean of  $\{\mathbf{f}_t\}$  is 0 for



technical convenience. Moreover,

$$\begin{aligned} \left\| \sum_{l=1}^p \hat{\mathbf{A}}_{l,p} \frac{1}{T-p} \sum_{t=p+1}^T \hat{\mathbf{f}}_{t-l} \right\| &\leq \sum_{l=1}^p \left\| \hat{\mathbf{A}}_{l,p} \right\|_F \left\| \frac{1}{T-p} \sum_{t=p+1}^T \hat{\mathbf{f}}_{t-l} \right\| \\ &= O_P(1) \times O_P \left( \frac{1}{\sqrt{T-p}} + \frac{1}{\sqrt{T}} + \frac{1}{\sqrt{N}} \right) = o_P(1), \end{aligned}$$

where the second last line follows from the summability conditions in Lemma C.5, the order of  $\|\hat{\mathbf{f}}_t - \mathbf{f}_t\|$  in Lemma C.3 and the fact that the mean of  $\{\hat{\mathbf{f}}_t\}$  is assumed to be 0 for technical convenience.

Lastly, we can show that  $\|\tilde{\mathbf{e}}_T\|^2 \rightarrow 0$  in probability with the same technique as stated above for  $\|\tilde{\mathbf{e}}_T\|$ . Hence with (10) and (11), we can conclude that  $\frac{1}{T} \sum_{t=1}^T \sum_{s=1}^T \|\mathcal{H}_{12}\|_F \rightarrow 0$  in probability. Together with the result that  $\frac{1}{T} \sum_{t=1}^T \sum_{s=1}^T \|\mathcal{H}_{11}\|_F \rightarrow 0$  in probability, we have  $\frac{1}{T} \sum_{t=1}^T \sum_{s=1}^T \|\mathcal{H}_1\|_F \rightarrow 0$  in probability. Therefore, it suffices to conclude that  $\mathcal{M}_3 \rightarrow 0$  in probability conditional on the sample.

Consequently, by utilizing Slutsky's theorem conditional on the sample, we can conclude that

$$d_K \left( \mathcal{L} \left( \sqrt{T} \mathbf{c}^\top \hat{\mathbf{Q}} (\bar{\mathbf{f}}_T^* - \mathbb{E}^* \bar{\mathbf{f}}_T^*) \mid \mathbf{y}_1, \mathbf{y}_2, \dots, \mathbf{y}_T \right), \mathcal{L} \left( \sqrt{T} \mathbf{c}^\top \mathbf{Q} (\bar{\mathbf{f}}_T - \mathbb{E} \bar{\mathbf{f}}_T) \right) \right) \xrightarrow{p} 0,$$

□

*Proof of Theorem 4.3.* Without loss of generality, we again assume  $\{\mathbf{f}_t\}$  are the demeaned factors (or the mean of factors are all 0) in this proof to simplify the notations.

Firstly, notice that  $\mathbf{f}_t^* = \sum_{l=1}^p \hat{\mathbf{A}}_{l,p} \mathbf{f}_{t-l}^* + \mathbf{e}_t^* = \sum_{l=1}^\infty \hat{\Psi}_{l,p} \mathbf{e}_{t-l}^* + \mathbf{e}_t^* = \sum_{l=0}^\infty \hat{\Psi}_{l,p} \mathbf{e}_{t-l}^*$ . We can then represent  $\mathbf{\Gamma}_f^*(k)$  as

$$\begin{aligned} \mathbf{\Gamma}_f^*(k) &= \text{Cov}^*(\mathbf{f}_t^*, \mathbf{f}_{t+k}^*) \\ &= \text{Cov}^* \left( \sum_{l_1=0}^\infty \hat{\Psi}_{l_1,p} \mathbf{e}_{t-l_1}^*, \sum_{l_2=0}^\infty \hat{\Psi}_{l_2,p} \mathbf{e}_{t+k-l_2}^* \right) \\ &= \sum_{l_1=0}^\infty \sum_{l_2=0}^\infty \hat{\Psi}_{l_1,p} \text{Cov}^*(\mathbf{e}_{t-l_1}^*, \mathbf{e}_{t+k-l_2}^*) \hat{\Psi}_{l_2,p}^\top \\ &= \sum_{l_1=0}^\infty \hat{\Psi}_{l_1,p} \text{Cov}^*(\mathbf{e}_{t-l_1}^*, \mathbf{e}_{t-l_1}^*) \hat{\Psi}_{l_1+k,p}^\top \\ &= \sum_{l=0}^\infty \hat{\Psi}_{l,p} \hat{\Sigma}_{e,p} \hat{\Psi}_{l+k,p}^\top \end{aligned}$$

where we stress the fact that  $\text{Cov}^*(\mathbf{e}_{t-l_1}^*, \mathbf{e}_{t-l_2}^*) = 0$  for  $l_1 \neq l_2$  and  $\text{Cov}^*(\mathbf{e}_{t-l_1}^*, \mathbf{e}_{t-l_1}^*) =$

$\mathbb{E}^*(e_t^* e_t^{*\top}) = \widehat{\Sigma}_{e,p}$  for all  $l_1 \in \mathbf{Z}$ , since  $e_t^*$  is uniformly distributed on the set of centered residuals  $(\widehat{e}_{t,p} - \widehat{e}_T)$ . Similarly,

$$\begin{aligned}\Gamma_f(k) &= \text{Cov}(\mathbf{f}_t, \mathbf{f}_{t+k}) \\ &= \text{Cov}\left(\sum_{l_1=0}^{\infty} \Psi_{l_1} e_{t-l_1}, \sum_{l_2=0}^{\infty} \Psi_{l_2} e_{t+k-l_2}\right) \\ &= \sum_{l_1=0}^{\infty} \sum_{l_2=0}^{\infty} \Psi_{l_1} \text{Cov}(e_{t-l_1}, e_{t+k-l_2}) \Psi_{l_2}^\top \\ &= \sum_{l_1=0}^{\infty} \Psi_{l_1} \text{Cov}(e_{t-l_1}, e_{t-l_1}) \Psi_{l_1+k}^\top \\ &= \sum_{l=0}^{\infty} \Psi_l \Sigma_e \Psi_{l+k}^\top,\end{aligned}$$

where we write  $\Sigma_e = \text{Cov}(e_t, e_t)$  and use the fact that  $\mathbf{f}_t = \sum_{l=1}^{\infty} \mathbf{A}_l \mathbf{f}_{t-l} + e_t = \sum_{l=1}^{\infty} \Psi_l e_{t-l} + e_t = \sum_{l=0}^{\infty} \Psi_l e_{t-l}$ .

To see the assertion in this theorem, we first of all define an intermediate term  $\Gamma_{f,p}(k) := \sum_{l=0}^{\infty} \Psi_{l,p} \Sigma_{e,p} \Psi_{l+k,p}^\top$ , where  $\{\Psi_{l,p}, l \in \mathbf{N}\}$  are the power series coefficients matrices of  $(\mathbf{I}_r - \sum_{l=1}^p \mathbf{A}_{l,p} z^l)^{-1}$  for  $|z| \leq 1$ , and  $\Sigma_{e,p} = \text{Cov}(e_{t,p}, e_{t,p})$  where  $e_{t,p} = \mathbf{f}_t - \sum_{l=1}^p \mathbf{A}_{l,p} \mathbf{f}_{t-l}$  with  $\{\mathbf{A}_{l,p}, l \in \mathbf{N}\}$  the finite predictor coefficients matrices of  $\{\mathbf{A}_l, l \in \mathbf{N}\}$ . Hence by triangular inequality, we have

$$\left\| \Gamma_f^*(k) - \Gamma_f(k) \right\|_2 \leq \left\| \Gamma_f^*(k) - \Gamma_{f,p}(k) \right\|_2 + \left\| \Gamma_{f,p}(k) - \Gamma_f(k) \right\|_2.$$

It is then sufficient to show both terms on the right side converge to 0 in probability. For  $\left\| \Gamma_f^*(k) - \Gamma_{f,p}(k) \right\|_2$ , we have

$$\begin{aligned}\left\| \Gamma_f^*(k) - \Gamma_{f,p}(k) \right\|_2 &= \left\| \sum_{l=0}^{\infty} \widehat{\Psi}_{l,p} \widehat{\Sigma}_{e,p} \widehat{\Psi}_{l+k,p}^\top - \sum_{l=0}^{\infty} \Psi_{l,p} \Sigma_{e,p} \Psi_{l+k,p}^\top \right\|_2 \\ &= \left\| \sum_{l=0}^{\infty} \left[ (\widehat{\Psi}_{l,p} - \Psi_{l,p}) \widehat{\Sigma}_{e,p} \widehat{\Psi}_{l+k,p}^\top + \Psi_{l,p} (\widehat{\Sigma}_{e,p} - \Sigma_{e,p}) \widehat{\Psi}_{l+k,p}^\top \right. \right. \\ &\quad \left. \left. + \Psi_{l,p} \Sigma_{e,p} (\widehat{\Psi}_{l+k,p} - \Psi_{l+k,p})^\top \right] \right\|_2 \\ &= O_P \left( \sum_{l=1}^{\infty} \left\| \widehat{\Psi}_{l,p} - \Psi_{l,p} \right\|_F \right) + O_P \left( \left\| \widehat{\Sigma}_{e,p} - \Sigma_{e,p} \right\|_F \right),\end{aligned}$$

where the second last line follows from the norm summable conditions on  $\widehat{\Psi}_{l,p}$  and  $\Psi_{l,p}$ . Hence we can use the results of Lemma C.7 and C.8 to conclude that  $\left\| \Gamma_f^*(k) - \Gamma_{f,p}(k) \right\|_2 \rightarrow 0$  in

probability. Similarly, we have

$$\begin{aligned}
\|\Gamma_{f,p}(k) - \Gamma_f(k)\|_2 &= \left\| \sum_{l=0}^{\infty} \Psi_{l,p} \Sigma_{e,p} \Psi_{l+k,p}^\top - \sum_{l=0}^{\infty} \Psi_l \Sigma_e \Psi_{l+k}^\top \right\|_2 \\
&= \left\| \sum_{l=0}^{\infty} \left[ (\Psi_{l,p} - \Psi_l) \Sigma_{e,p} \Psi_{l+k,p}^\top + \Psi_l (\Sigma_{e,p} - \Sigma_e) \Psi_{l+k,p}^\top \right. \right. \\
&\quad \left. \left. + \Psi_l \Sigma_e (\Psi_{l+k,p} - \Psi_{l+k})^\top \right] \right\|_2 \\
&= O_P \left( \sum_{l=1}^{\infty} \|\Psi_{l,p} - \Psi_l\|_F \right) + O_P (\|\Sigma_{e,p} - \Sigma_e\|_F),
\end{aligned}$$

since  $\Psi_{l,p}$  and  $\Psi_l$  are norm summable. Hence  $\|\Gamma_{f,p}(k) - \Gamma_f(k)\|_2 \rightarrow 0$  in probability by Lemmas C.7 and C.8. Therefore we can conclude that  $\|\Gamma_f^*(k) - \Gamma_f(k)\|_2 \rightarrow 0$  in probability.  $\square$

*Proof of Proposition 4.4.* To see the assertions, we first note that,

$$\begin{aligned}
\|\Gamma_y^*(k) - \Gamma_y(k)\|_2 &= \left\| \widehat{Q} \Gamma_f^*(k) \widehat{Q}^T - Q \Gamma_f(k) Q^T \right\|_2 \\
&\leq \left\| (\widehat{Q} - Q) \Gamma_f^*(k) \widehat{Q}^T \right\|_2 + \left\| Q (\Gamma_f^*(k) - \Gamma_f(k)) \widehat{Q}^T \right\|_2 \\
&\quad + \left\| Q \Gamma_f(k) (\widehat{Q} - Q)^T \right\|_2 \\
&= O_P \left( N^{1/2} \|\widehat{Q} - Q\|_2 \right) + O_P \left( N \|\Gamma_f^*(k) - \Gamma_f(k)\|_2 \right) = o_P(1),
\end{aligned}$$

where the last line follows from Assumption 3.1, Lemma C.1 and Theorem 4.3. To see that  $|\delta_i^*(k) - \delta_i(k)| \xrightarrow{P} 0$  for  $N \rightarrow \infty$  and  $T \rightarrow \infty$ , we can apply Weyl's Eigenvalue Theorem (Fan et al. 2013), that is

$$|\delta_i^*(k) - \delta_i(k)| \leq \frac{1}{N^2} \left\| \Gamma_y^*(k) \Gamma_y^*(k)^\top - \Gamma_y(k) \Gamma_y(k)^\top \right\|_2.$$

Furthermore,

$$\begin{aligned}
\frac{1}{N^2} \left\| \Gamma_y^*(k) \Gamma_y^*(k)^\top - \Gamma_y(k) \Gamma_y(k)^\top \right\|_2 &= \frac{1}{N^2} \left\| \left[ \Gamma_y^*(k) - \Gamma_y(k) \right] \Gamma_y^*(k)^\top + \Gamma_y(k) \left[ \Gamma_y^*(k) - \Gamma_y(k) \right]^\top \right\|_2 \\
&\leq \frac{1}{N^2} \left\| \left[ \Gamma_y^*(k) - \Gamma_y(k) \right] \Gamma_y^*(k)^\top \right\|_2 \\
&\quad + \frac{1}{N^2} \left\| \Gamma_y(k) \left[ \Gamma_y^*(k) - \Gamma_y(k) \right]^\top \right\|_2.
\end{aligned}$$

It is then sufficient to consider one of the two terms on the right side since the other one can be dealt with similarly. To study  $\frac{1}{N^2} \left\| \left[ \Gamma_y^*(k) - \Gamma_y(k) \right] \Gamma_y^*(k)^\top \right\|_2$ , we first notice that from Assumption 3.1, Lemma C.1 and Theorem 4.3,  $\|\Gamma_y^*(k)\|_2 = \|\widehat{Q} \Gamma_f^*(k) \widehat{Q}^T\|_2 \asymp N$ . Therefore, we

have

$$\begin{aligned} \frac{1}{N^2} \left\| \left[ \mathbf{\Gamma}_y^*(k) - \mathbf{\Gamma}_y(k) \right] \mathbf{\Gamma}_y^*(k)^\top \right\|_2 &= O_P \left( \frac{1}{N} \left\| \mathbf{\Gamma}_y^*(k) - \mathbf{\Gamma}_y(k) \right\|_2 \right) \\ &= O_P \left( N^{-1/2} \left\| \hat{\mathbf{Q}} - \mathbf{Q} \right\|_2 \right) + O_P \left( \left\| \mathbf{\Gamma}_f^*(k) - \mathbf{\Gamma}_f(k) \right\|_2 \right), \end{aligned}$$

where both terms on the right side converge to 0 in probability as shown in Lemma C.2 and Theorem 4.3.  $\square$

## C Auxiliary lemmas and proofs

In this section, we present some auxiliary results that facilitate the proofs of theorems in this paper. Those auxiliary results are divided into two subsections according to the related topics. In the first subsection, we present some results for factor models' estimates, and in the second subsection, the results for AR-sieve bootstrap of factor models are summarised.

### C.1 Auxiliary results for estimates of factor models

**Lemma C.1.** Denoted by  $\|\mathbf{V}\|_{\min}$  the positive square root of the minimum eigenvalue of  $\mathbf{V}\mathbf{V}^\top$  or  $\mathbf{V}^\top\mathbf{V}$ , under Assumption 3.1, we have

$$\left\| \mathbf{\Gamma}_f(k) \right\|_2 \asymp 1 \asymp \left\| \mathbf{\Gamma}_f(k) \right\|_{\min},$$

and

$$\left\| \tilde{\mathbf{\Gamma}}_f(k) - \mathbf{\Gamma}_f(k) \right\|_2 = O_P \left( T^{-1/2} \right).$$

Lemma C.1 is a modification of the results in Lemma 1 and 2 of Lam et al. (2011) for the strong factors' case, since we have assumed  $\mathbf{Q}^\top \mathbf{Q} = N\mathbf{I}_r$  but not  $\mathbf{Q}^\top \mathbf{Q} = \mathbf{I}_r$  as in Lam et al. (2011). Therefore, the proof of Lemma C.1 is similar to the proofs of Lemma 1 and 2 in Lam et al. (2011), hence omitted.

**Lemma C.2.** Under Assumption 3.1,

$$\left\| \hat{\mathbf{Q}} - \mathbf{Q} \right\|_2 = O_P \left( N^{1/2} T^{-1/2} \right),$$

and

$$N^{-1/2} \left\| \hat{\mathbf{Q}} \hat{\mathbf{f}}_t - \mathbf{Q} \mathbf{f}_t \right\|_2 = O_P \left( T^{-1/2} + N^{-1/2} \right).$$

Although compared with the model introduced in [Lam et al. \(2011\)](#), we scale the columns in  $\mathbf{Q}$  by  $\sqrt{N}$  in our factor models' setting, the above convergence rate is the same as that of strong factors' case in Theorem 3 of [Lam et al. \(2011\)](#). Besides, the proof of Lemma C.2 is the case for strong factors in the proof of Theorem 3 in [Lam et al. \(2011\)](#) with the only difference on scaled factor loading matrix  $\mathbf{Q}$  and factors  $\mathbf{f}$ . Therefore, the proof is omitted here.

**Lemma C.3.** Define  $\hat{\Gamma}_f(k) = \frac{1}{T-k} \sum_{t=1}^{T-k} \hat{\mathbf{f}}_t \hat{\mathbf{f}}_{t+k}^\top$  and  $\tilde{\Gamma}_f(k) = \frac{1}{T-k} \sum_{t=1}^{T-k} \mathbf{f}_t \mathbf{f}_{t+k}^\top$ , for some  $k \leq p$ , where  $p$  fulfils Assumption 4.3. It then holds that

$$\left\| \hat{\Gamma}_f(k) - \tilde{\Gamma}_f(k) \right\|_2 = O_P \left( N^{-1/2} + T^{-1/2} \right).$$

Lemma C.3 illustrates the convergence rate on autocovariance matrices of estimated factors under strong factors' case, which is an extension to the convergence rate of estimated factors obtained in Theorem 3 in [Lam et al. \(2011\)](#).

*Proof of Lemma C.3.* First of all, we notice that

$$\begin{aligned} \hat{\Gamma}_f(k) - \tilde{\Gamma}_f(k) &= \frac{1}{T-k} \sum_{t=1}^{T-k} \left( \hat{\mathbf{f}}_t \hat{\mathbf{f}}_{t+k}^\top - \mathbf{f}_t \mathbf{f}_{t+k}^\top \right) \\ &= \frac{1}{T-k} \sum_{t=1}^{T-k} \left[ \left( \hat{\mathbf{f}}_t - \mathbf{f}_t \right) \hat{\mathbf{f}}_{t+k}^\top + \mathbf{f}_t \left( \hat{\mathbf{f}}_{t+k} - \mathbf{f}_{t+k} \right)^\top \right]. \end{aligned}$$

Hence,

$$\begin{aligned} \left\| \hat{\Gamma}_f(k) - \tilde{\Gamma}_f(k) \right\|_2 &\leq \left\| \frac{1}{T-k} \sum_{t=1}^{T-k} \left( \hat{\mathbf{f}}_t - \mathbf{f}_t \right) \hat{\mathbf{f}}_{t+k}^\top \right\|_2 + \left\| \frac{1}{T-k} \sum_{t=1}^{T-k} \mathbf{f}_t \left( \hat{\mathbf{f}}_{t+k} - \mathbf{f}_{t+k} \right)^\top \right\|_2 \\ &\leq \frac{1}{T-k} \sum_{t=1}^{T-k} \left\| \left( \hat{\mathbf{f}}_t - \mathbf{f}_t \right) \hat{\mathbf{f}}_{t+k}^\top \right\|_2 + \frac{1}{T-k} \sum_{t=1}^{T-k} \left\| \mathbf{f}_t \left( \hat{\mathbf{f}}_{t+k} - \mathbf{f}_{t+k} \right)^\top \right\|_2. \end{aligned}$$

And it is sufficient to consider only one of the two terms on the right-hand side above since the other one can be dealt with in precisely the same way. For the first term on the right-hand side above, notice that under the factor model defined in (3), we have

$$\begin{aligned} \hat{\mathbf{f}}_t - \mathbf{f}_t &= \frac{1}{N} \hat{\mathbf{Q}}^\top \mathbf{y}_t - \mathbf{f}_t \\ &= \frac{1}{N} \left( \hat{\mathbf{Q}} - \mathbf{Q} \right)^\top \mathbf{y}_t + \frac{1}{N} \mathbf{Q}^\top \mathbf{y}_t - \mathbf{f}_t \\ &= \frac{1}{N} \left( \hat{\mathbf{Q}} - \mathbf{Q} \right)^\top \mathbf{y}_t + \frac{1}{N} \mathbf{Q}^\top \mathbf{y}_t - \frac{1}{N} \mathbf{Q}^\top \mathbf{Q} \mathbf{f}_t \\ &= \frac{1}{N} \left( \hat{\mathbf{Q}} - \mathbf{Q} \right)^\top \mathbf{y}_t + \frac{1}{N} \mathbf{Q}^\top \mathbf{u}_t. \end{aligned}$$

Hence

$$\left\| \hat{\mathbf{f}}_t - \mathbf{f}_t \right\|_2 \leq \left\| \frac{1}{N} (\hat{\mathbf{Q}} - \mathbf{Q})^\top \mathbf{y}_t \right\|_2 + \left\| \frac{1}{N} \mathbf{Q}^\top \mathbf{u}_t \right\|_2,$$

by triangular inequality. To study  $\left\| \frac{1}{N} \mathbf{Q}^\top \mathbf{u}_t \right\|_2$ , first consider the random variables  $\frac{1}{\sqrt{N}} \mathbf{q}_i^\top \mathbf{u}_t$  for each  $\frac{1}{\sqrt{N}} \mathbf{q}_i$  in  $\frac{1}{\sqrt{N}} \mathbf{Q} = \left( \frac{1}{\sqrt{N}} \mathbf{q}_1, \frac{1}{\sqrt{N}} \mathbf{q}_2, \dots, \frac{1}{\sqrt{N}} \mathbf{q}_r \right)$ , where  $\frac{1}{\sqrt{N}} \mathbf{q}_i$  for  $i = 1, 2, \dots, r$  are unscaled eigenvectors estimated from  $\hat{\mathbf{L}}$ . Observe that  $\mathbb{E} \left( \frac{1}{\sqrt{N}} \mathbf{q}_i^\top \mathbf{u}_t \right) = 0$  and  $\mathbb{V} \left( \frac{1}{\sqrt{N}} \mathbf{q}_i^\top \mathbf{u}_t \right) = \frac{1}{N} \mathbf{q}_i^\top \boldsymbol{\Sigma}_u \mathbf{q}_i \leq \lambda_{\max}(\boldsymbol{\Sigma}_u) < \infty$ , since  $\left\| \frac{1}{\sqrt{N}} \mathbf{q}_i \right\|_2 = 1$  and  $\lambda_{\max}(\boldsymbol{\Sigma}_u)$  is the largest eigenvalue of  $\boldsymbol{\Sigma}_u$ . Consequently,  $\frac{1}{\sqrt{N}} \mathbf{q}_i^\top \mathbf{u}_t = O_P(1)$  and  $\left\| \frac{1}{N} \mathbf{Q}^\top \mathbf{u}_t \right\|_2 = \sqrt{\frac{1}{N} \sum_{i=1}^r \left( \frac{1}{\sqrt{N}} \mathbf{q}_i^\top \mathbf{u}_t \right)^2} = O_P(N^{-1/2})$ , as the eigenvalues of  $\boldsymbol{\Sigma}_u$  are assumed to be bounded when  $N \rightarrow \infty$  under Assumption 3.1.

Recall that  $\left\| \hat{\mathbf{Q}} - \mathbf{Q} \right\|_2 = O_P(N^{1/2} T^{-1/2})$  by Lemma C.2, we then have  $\left\| \frac{1}{N} (\hat{\mathbf{Q}} - \mathbf{Q})^\top \mathbf{y}_t \right\|_2 \leq \frac{1}{N} \left\| (\hat{\mathbf{Q}} - \mathbf{Q})^\top \right\|_2 \left\| \mathbf{y}_t \right\|_2 = O_P(T^{-1/2})$ , and

$$\begin{aligned} \left\| \hat{\mathbf{f}}_t - \mathbf{f}_t \right\|_2 &\leq \left\| \frac{1}{N} (\hat{\mathbf{Q}} - \mathbf{Q})^\top \mathbf{y}_t \right\|_2 + \left\| \frac{1}{N} \mathbf{Q}^\top \mathbf{u}_t \right\|_2 \\ &= O_P(N^{-1/2} + T^{-1/2}), \end{aligned}$$

uniformly for  $t$ . Finally, we can conclude that

$$\begin{aligned} \left\| \hat{\Gamma}_f(k) - \tilde{\Gamma}_f(k) \right\|_2 &\leq \frac{1}{T-k} \sum_{t=1}^{T-k} \left\| (\hat{\mathbf{f}}_t - \mathbf{f}_t) \hat{\mathbf{f}}_{t+k}^\top \right\|_2 + \frac{1}{T-k} \sum_{t=1}^{T-k} \left\| \mathbf{f}_t (\hat{\mathbf{f}}_{t+k} - \mathbf{f}_{t+k})^\top \right\|_2 \\ &= O_P(N^{-1/2} + T^{-1/2}). \end{aligned}$$

□

## C.2 Auxiliary results for AR-sieve bootstrap of factor models

**Lemma C.4.** Let  $\tilde{\mathbf{A}}_p = \left( \tilde{\mathbf{A}}_{1,p}, \tilde{\mathbf{A}}_{2,p}, \dots, \tilde{\mathbf{A}}_{p,p} \right)$  be the matrix of the Yule-Walker estimators of the finite predictor coefficients on true factors  $\{\mathbf{f}_t\}$ , and  $\hat{\mathbf{A}}_p = \left( \hat{\mathbf{A}}_{1,p}, \hat{\mathbf{A}}_{2,p}, \dots, \hat{\mathbf{A}}_{p,p} \right)$  be the matrix of the Yule-Walker estimators of the finite predictor coefficients on estimated factors  $\{\hat{\mathbf{f}}_t\}$ , then

$$\left\| \hat{\mathbf{A}}_p - \tilde{\mathbf{A}}_p \right\|_F = O_P(p^4 (N^{-1/2} + T^{-1/2})).$$

*Proof of Lemma C.4.* Recall that the Yule-Walker estimators are solved from the Yule-Walker

equations on the finite predictors' coefficients matrices as follows,

$$\mathbf{A}_p = (\mathbf{A}_{1,p}, \mathbf{A}_{2,p}, \dots, \mathbf{A}_{p,p}) = \mathbf{\Pi}_1 \mathbf{\Pi}_{0,p}^{-1}$$

where  $\mathbf{\Pi}_1 = (\mathbf{\Gamma}_f(1), \mathbf{\Gamma}_f(2), \dots, \mathbf{\Gamma}_f(p))$  is an  $r \times (rp)$  block matrix of autocovariance matrices and

$$\mathbf{\Pi}_{0,p} = \begin{pmatrix} \mathbf{\Gamma}_f(0) & \mathbf{\Gamma}_f(1) & \cdots & \mathbf{\Gamma}_f(p-1) \\ \mathbf{\Gamma}_f(-1) & \mathbf{\Gamma}_f(0) & \cdots & \mathbf{\Gamma}_f(p-2) \\ \vdots & \vdots & \ddots & \vdots \\ \mathbf{\Gamma}_f(-p+1) & \mathbf{\Gamma}_f(-p+2) & \cdots & \mathbf{\Gamma}_f(0) \end{pmatrix},$$

is then an  $(rp) \times (rp)$  block matrix of autocovariance matrices (Brockwell & Davis 1991). Write  $\hat{\mathbf{A}}_p = (\hat{\mathbf{A}}_{1,p}, \hat{\mathbf{A}}_{2,p}, \dots, \hat{\mathbf{A}}_{p,p}) = \hat{\mathbf{\Pi}}_1 \hat{\mathbf{\Pi}}_{0,p}^{-1}$  with  $\hat{\mathbf{\Pi}}_1$  and  $\hat{\mathbf{\Pi}}_{0,p}$  the same matrices as  $\mathbf{\Pi}_1$  and  $\mathbf{\Pi}_{0,p}$  but defined based on  $\hat{\mathbf{\Gamma}}_f$  rather than  $\mathbf{\Gamma}_f$ . Similarly,  $\tilde{\mathbf{A}}_p = (\tilde{\mathbf{A}}_{1,p}, \tilde{\mathbf{A}}_{2,p}, \dots, \tilde{\mathbf{A}}_{p,p}) = \tilde{\mathbf{\Pi}}_1 \tilde{\mathbf{\Pi}}_{0,p}^{-1}$  with  $\tilde{\mathbf{\Pi}}_1$  and  $\tilde{\mathbf{\Pi}}_{0,p}$  defined based on  $\tilde{\mathbf{\Gamma}}_f$  rather than  $\mathbf{\Gamma}_f$ . Recall that  $\hat{\mathbf{\Gamma}}_f$  and  $\tilde{\mathbf{\Gamma}}_f$  are sample lag- $k$  autocovariance matrices defined in Lemma C.3, then we have

$$\|\hat{\mathbf{A}}_p - \tilde{\mathbf{A}}_p\|_F \leq \|\hat{\mathbf{\Pi}}_{0,p}^{-1} - \tilde{\mathbf{\Pi}}_{0,p}^{-1}\|_F \|\hat{\mathbf{\Pi}}_1\|_F + \|\tilde{\mathbf{\Pi}}_{0,p}^{-1}\|_F \|\hat{\mathbf{\Pi}}_1 - \tilde{\mathbf{\Pi}}_1\|_F. \quad (12)$$

To find  $\|\tilde{\mathbf{\Pi}}_{0,p}^{-1}\|_F$ , we first compute  $\|\mathbf{\Pi}_{0,p}^{-1}\|_F$ . Recall the recursive derivation based on the partitioned inverse formula for  $\mathbf{\Pi}_{0,p+1}^{-1}$  as in Sowell (1989),

$$\begin{aligned} \mathbf{\Pi}_{0,p+1}^{-1} &= \begin{pmatrix} \mathbf{\Pi}_{0,p}^{-1} + \mathcal{J}_p \bar{\mathbf{A}}_p \bar{\mathbf{v}}_p^{-1} \bar{\mathbf{A}}_p^\top \mathcal{J}_p & -\mathcal{J}_p \bar{\mathbf{A}}_p \bar{\mathbf{v}}_p^{-1} \\ -\bar{\mathbf{v}}_p^{-1} \bar{\mathbf{A}}_p^\top \mathcal{J}_p & \bar{\mathbf{v}}_p^{-1} \end{pmatrix} \\ &= \begin{pmatrix} \mathbf{\Pi}_{0,p}^{-1} & 0 \\ 0 & 0 \end{pmatrix} + \begin{pmatrix} 0 & -\mathcal{J}_p \bar{\mathbf{A}}_p \bar{\mathbf{v}}_p^{-1/2} \\ 0 & \bar{\mathbf{v}}_p^{-1/2} \end{pmatrix} \begin{pmatrix} 0 & 0 \\ -\bar{\mathbf{v}}_p^{-1/2} \bar{\mathbf{A}}_p^\top \mathcal{J}_p & \bar{\mathbf{v}}_p^{-1/2} \end{pmatrix}, \end{aligned} \quad (13)$$

where  $\mathcal{J}_p = \mathbf{J}_p \otimes \mathbf{I}_r$  with  $\mathbf{J}_p$  the  $p \times p$  matrix with ones on the anti-diagonal and  $\mathbf{I}_r$  the  $r \times r$  identity matrix,  $\bar{\mathbf{v}} = \mathbb{E}(\mathbf{f}_t - \sum_{l=1}^p \bar{\mathbf{A}}_{l,p} \mathbf{f}_{t+l}) (\mathbf{f}_t - \sum_{l=1}^p \bar{\mathbf{A}}_{l,p} \mathbf{f}_{t+l})^\top$  and  $\bar{\mathbf{A}}_p = (\bar{\mathbf{A}}_{1,p}^\top, \bar{\mathbf{A}}_{2,p}^\top, \dots, \bar{\mathbf{A}}_{p,p}^\top)$  the coefficient matrices minimizing the forward prediction variance  $\mathbb{E}(\mathbf{f}_t - \sum_{l=1}^p \mathbf{F}_{l,p} \mathbf{f}_{t+l}) (\mathbf{f}_t - \sum_{l=1}^p \mathbf{F}_{l,p} \mathbf{f}_{t+l})^\top$ . Denoted by  $\mathcal{S}_p$  the second term on the right-hand side of (13), we can then get the recursive expression of  $\mathbf{\Pi}_{0,p}^{-1}$  as

$$\mathbf{\Pi}_{0,p}^{-1} = \begin{pmatrix} \mathbf{\Gamma}_f(0)^{-1} & 0 \\ 0 & 0 \end{pmatrix} + \sum_{l=1}^{p-1} \mathcal{S}_l.$$

For  $\mathcal{S}_l$ , note that

$$\begin{aligned}\|\mathcal{S}_l\|_F &\leq \left\|\bar{\mathbf{v}}_l^{-1/2}\right\|_F^2 (1 + \|\mathcal{J}_l \bar{\mathbf{A}}_l\|_F)^2 \\ &\leq \left\|\bar{\mathbf{v}}_l^{-1/2}\right\|_F^2 \left(1 + \sum_{j=1}^l \|\bar{\mathbf{A}}_{j,l}\|_F\right)^2 \\ &= O(1),\end{aligned}$$

uniformly for  $l = 1, 2, \dots, p$ , where we use the definition of  $\bar{\mathbf{v}}_l$  and Lemma C.5. Hence  $\left\|\sum_{l=1}^{p-1} \mathcal{S}_l\right\|_F \leq \sum_{l=1}^{p-1} \|\mathcal{S}_l\|_F = O(p)$ . Besides,  $\|\mathbf{\Gamma}_f(0)^{-1}\|_F = \sqrt{\sum_{i=1}^r \lambda_i^{-2}} \leq \sqrt{r} \lambda_{\min}^{-1} = O(1)$ , where  $\lambda_i$  is the  $i^{\text{th}}$  eigenvalue of  $\mathbf{\Gamma}_f(0)$ ,  $\lambda_{\min}$  is the smallest eigenvalue of  $\mathbf{\Gamma}_f(0)$  and we use Assumption 4.1 that  $\mathbf{\Gamma}_f(0)$  is full rank. Thus, we have shown  $\left\|\mathbf{\Pi}_{0,p}^{-1}\right\|_F = O(p)$ .

To find  $\left\|\hat{\mathbf{\Pi}}_{0,p}^{-1} - \tilde{\mathbf{\Pi}}_{0,p}^{-1}\right\|_F$ , note that for invertible matrices  $\hat{\mathbf{\Pi}}_{0,p}$  and  $\tilde{\mathbf{\Pi}}_{0,p}$ ,

$$\begin{aligned}\left\|\hat{\mathbf{\Pi}}_{0,p}^{-1} - \tilde{\mathbf{\Pi}}_{0,p}^{-1}\right\|_F &= \left\|\hat{\mathbf{\Pi}}_{0,p}^{-1}(\tilde{\mathbf{\Pi}}_{0,p} - \hat{\mathbf{\Pi}}_{0,p})\tilde{\mathbf{\Pi}}_{0,p}^{-1}\right\|_F \\ &= \left\|(\hat{\mathbf{\Pi}}_{0,p}^{-1} - \tilde{\mathbf{\Pi}}_{0,p}^{-1})(\tilde{\mathbf{\Pi}}_{0,p} - \hat{\mathbf{\Pi}}_{0,p})\tilde{\mathbf{\Pi}}_{0,p}^{-1} + \tilde{\mathbf{\Pi}}_{0,p}^{-1}(\tilde{\mathbf{\Pi}}_{0,p} - \hat{\mathbf{\Pi}}_{0,p})\tilde{\mathbf{\Pi}}_{0,p}^{-1}\right\|_F \\ &\leq \left\|\hat{\mathbf{\Pi}}_{0,p}^{-1} - \tilde{\mathbf{\Pi}}_{0,p}^{-1}\right\|_F \left\|\tilde{\mathbf{\Pi}}_{0,p} - \hat{\mathbf{\Pi}}_{0,p}\right\|_F \left\|\tilde{\mathbf{\Pi}}_{0,p}^{-1}\right\|_F + \left\|\tilde{\mathbf{\Pi}}_{0,p} - \hat{\mathbf{\Pi}}_{0,p}\right\|_F \left\|\tilde{\mathbf{\Pi}}_{0,p}^{-1}\right\|_F^2.\end{aligned}$$

And for large enough  $N$  and  $T$  such as  $\left\|\hat{\mathbf{\Gamma}}_f(k) - \tilde{\mathbf{\Gamma}}_f(k)\right\|_2 \rightarrow 0$  and  $\left\|\tilde{\mathbf{\Pi}}_{0,p} - \hat{\mathbf{\Pi}}_{0,p}\right\|_F \rightarrow 0$  in probability, we can write

$$\begin{aligned}\left\|\hat{\mathbf{\Pi}}_{0,p}^{-1} - \tilde{\mathbf{\Pi}}_{0,p}^{-1}\right\|_F &\leq \frac{\left\|\tilde{\mathbf{\Pi}}_{0,p}^{-1}\right\|_F^2 \left\|\tilde{\mathbf{\Pi}}_{0,p} - \hat{\mathbf{\Pi}}_{0,p}\right\|_F}{1 - \left\|\tilde{\mathbf{\Pi}}_{0,p}^{-1}\right\|_F \left\|\tilde{\mathbf{\Pi}}_{0,p} - \hat{\mathbf{\Pi}}_{0,p}\right\|_F} \\ &\leq \frac{\left\|\mathbf{\Pi}_{0,p}^{-1}\right\|_F^2 \left\|\tilde{\mathbf{\Pi}}_{0,p} - \hat{\mathbf{\Pi}}_{0,p}\right\|_F}{1 - \left\|\tilde{\mathbf{\Pi}}_{0,p}^{-1}\right\|_F \left\|\tilde{\mathbf{\Pi}}_{0,p} - \hat{\mathbf{\Pi}}_{0,p}\right\|_F} + \frac{\left\|\tilde{\mathbf{\Pi}}_{0,p}^{-1} - \mathbf{\Pi}_{0,p}^{-1}\right\|_F^2 \left\|\tilde{\mathbf{\Pi}}_{0,p} - \hat{\mathbf{\Pi}}_{0,p}\right\|_F}{1 - \left\|\tilde{\mathbf{\Pi}}_{0,p}^{-1}\right\|_F \left\|\tilde{\mathbf{\Pi}}_{0,p} - \hat{\mathbf{\Pi}}_{0,p}\right\|_F} \\ &= O_P\left(\left\|\mathbf{\Pi}_{0,p}^{-1}\right\|_F^2 \left\|\tilde{\mathbf{\Pi}}_{0,p} - \hat{\mathbf{\Pi}}_{0,p}\right\|_F\right),\end{aligned}$$

where the last line follows since when  $N, T \rightarrow \infty$ ,  $\left\|\tilde{\mathbf{\Pi}}_{0,p} - \hat{\mathbf{\Pi}}_{0,p}\right\|_F \rightarrow 0$  in probability and the first term in the second last line is the leading term. In addition, we have

$$\begin{aligned}\left\|\tilde{\mathbf{\Pi}}_{0,p} - \hat{\mathbf{\Pi}}_{0,p}\right\|_F &\leq \sum_{l=1}^p \sum_{j=1}^p \left\|\hat{\mathbf{\Gamma}}_f(l-j) - \tilde{\mathbf{\Gamma}}_f(l-j)\right\|_F \\ &\leq p^2 \max_{|k| \leq p-1} \left\|\hat{\mathbf{\Gamma}}_f(k) - \tilde{\mathbf{\Gamma}}_f(k)\right\|_F \\ &= O_P\left(p^{5/2} \left(N^{-1/2} + T^{-1/2}\right)\right),\end{aligned}\tag{14}$$



where for  $r \times r$  matrices  $\widehat{\Gamma}_f(k)$  and  $\widetilde{\Gamma}_f(k)$ ,  $\left\| \widehat{\Gamma}_f(k) - \widetilde{\Gamma}_f(k) \right\|_F \asymp \left\| \widehat{\Gamma}_f(k) - \widetilde{\Gamma}_f(k) \right\|_2 = O_P(N^{-1/2} + T^{-1/2})$  as shown in Lemma C.3. Therefore, with (14) we can conclude that

$$\begin{aligned} \left\| \widehat{\Pi}_{0,p}^{-1} - \widetilde{\Pi}_{0,p}^{-1} \right\|_F &= O_P \left( \left\| \Pi_{0,p}^{-1} \right\|_F^2 \left\| \widetilde{\Pi}_{0,p} - \widehat{\Pi}_{0,p} \right\|_F \right) \\ &= O_P \left( p^4 \left( N^{-1/2} + T^{-1/2} \right) \right). \end{aligned} \quad (15)$$

Lastly,

$$\begin{aligned} \left\| \widehat{\Pi}_1 \right\|_F &\leq \sum_{k=1}^p \left\| \widehat{\Gamma}_f(k) \right\|_F \\ &\leq \sum_{k=1}^p \left\| \Gamma_f(k) \right\|_F + \sum_{k=1}^p \left\| \widehat{\Gamma}_f(k) - \Gamma_f(k) \right\|_F \\ &= O(1) + O_P \left( p \left( N^{-1/2} + T^{-1/2} \right) \right), \end{aligned} \quad (16)$$

where the first term follows from the summability condition in Assumption 4.1. Moreover,

$$\begin{aligned} \left\| \widehat{\Pi}_1 - \widetilde{\Pi}_1 \right\|_F &\leq \sum_{k=1}^p \left\| \widehat{\Gamma}_f(k) - \widetilde{\Gamma}_f(k) \right\|_F \\ &= O_P \left( p \left( N^{-1/2} + T^{-1/2} \right) \right). \end{aligned}$$

Hence we can conclude that the first term in (12) is the leading term, and

$$\left\| \widehat{\mathbf{A}}_p - \widetilde{\mathbf{A}}_p \right\|_F = O_P \left( p^4 \left( N^{-1/2} + T^{-1/2} \right) \right),$$

by (15) and (16). □

**Lemma C.5.** Let  $\{f_t\}$  be factor processes fulfilling Assumptions 3.1 and 4.1 for some  $\gamma \geq 0$ . Write  $\{\mathbf{A}_{l,p}, l = 1, 2, \dots, p\}$  and  $\{\Psi_{l,p}, l = 1, 2, \dots, p\}$  as the finite predictor coefficients matrices of the AR coefficients  $\{\mathbf{A}_l, l \in \mathbb{N}\}$  and the MA coefficients  $\{\Psi_l, l \in \mathbb{N}\}$  as in (3) and (2), respectively.

(i) Norm summability: the coefficients matrices  $\mathbf{A}_l$  and  $\Psi_l$  fulfil the following summability properties:

$$\sum_{l=1}^{\infty} (1+l)^\gamma \left\| \mathbf{A}_l \right\|_F < \infty \text{ and } \sum_{l=1}^{\infty} (1+l)^\gamma \left\| \Psi_l \right\|_F < \infty.$$

(ii) (Lemma 3.1 of Meyer & Kreiss (2015)) For some  $\gamma \geq 0$  as in Assumption 4.1, there exist  $p_0 \in \mathbb{N}$  and  $d < \infty$  such that

$$\sum_{l=1}^p (1+l)^\gamma \left\| \mathbf{A}_{l,p} - \mathbf{A}_l \right\|_F \leq d \sum_{l=p+1}^{\infty} (1+l)^\gamma \left\| \mathbf{A}_l \right\|_F, \text{ for } p \geq p_0,$$

and the right side converges to 0 when  $p \rightarrow \infty$ .

(iii) (Lemma 3.2 of [Meyer & Kreiss \(2015\)](#)) Let  $\mathbf{A}_p(z) := \mathbf{I}_r - \sum_{l=1}^p \mathbf{A}_{l,p} z^l$ , then there exist  $p_1 \in \mathbb{N}$  and  $c < \infty$  such that

$$\inf_{|z| \leq 1+1/p} |\det(\mathbf{A}_p(z))| \geq c, \text{ for } p \geq p_1.$$

(iv) (Lemma 3.3 of [Meyer & Kreiss \(2015\)](#)) Let  $\{\Psi_{l,p}, l \in \mathbb{N}\}$  be the power series coefficients matrices of  $(\mathbf{I}_r - \sum_{l=1}^p \mathbf{A}_{l,p} z^l)^{-1}$ , for  $|z| \leq 1$ . For  $p_1$  as defined in (iii) and some  $\gamma \geq 0$  in Assumption 4.1, there exist  $p_2 \geq p_1$  and  $d < \infty$  such that

$$\sum_{l=1}^{\infty} (1+l)^\gamma \|\Psi_{l,p} - \Psi_l\|_F \leq d \sum_{l=p+1}^{\infty} (1+l)^\gamma \|\mathbf{A}_l\|_F, \text{ for } p \geq p_2,$$

and the right side converges to 0 when  $p \rightarrow \infty$ .

Lemma C.5 (ii) is the vector form of Baxter's inequality on the AR coefficients matrices  $\{\mathbf{A}_l\}$  and its finite predictor coefficients matrices  $\{\mathbf{A}_{l,p}\}$ , whereas Lemma C.5 (iv) relates Baxter's inequality of AR coefficients to the MA coefficients matrices  $\{\Psi_l\}$  and its finite predictor coefficients matrices  $\{\Psi_{l,p}\}$ . The proofs of Lemma C.5 can be found in [Meyer & Kreiss \(2015\)](#), hence it is omitted here.

**Lemma C.6.** (Lemma 3.5 of [Meyer & Kreiss \(2015\)](#)) Let  $\{f_t\}$  be factor processes defined under the assumptions of Lemma C.5 and also fulfil Assumption 4.2. Define  $\Psi_{l,p}$  as the coefficients matrices in the power series of  $(\mathbf{I}_r - \sum_{l=1}^p \mathbf{A}_{l,p} z^l)^{-1}$ , for  $|z| \leq 1$  with  $\Psi_{0,q} := \mathbf{I}_r$  and  $\tilde{\Psi}_{l,p}$  as the power series coefficients matrices of  $(\mathbf{I}_r - \sum_{l=1}^p \tilde{\mathbf{A}}_{l,p} z^l)^{-1}$ , for  $|z| \leq 1$  with  $\tilde{\Psi}_{0,q} := \mathbf{I}_r$ . Then, there exists  $p_3 \in \mathbb{N}$  such that it holds uniformly in  $l \in \mathbb{N}$  and for all  $p \geq p_3$ ,

$$\|\tilde{\Psi}_{l,p} - \Psi_{l,p}\|_F \leq \left(1 + \frac{1}{p}\right)^{-l} \frac{1}{p^2} O_P(1).$$

The proof of Lemma C.6 can be found in [Meyer & Kreiss \(2015\)](#).

**Lemma C.7.** Let  $\{f_t\}$  be factor processes fulfilling Assumptions 3.1, 4.1 ( $\gamma = 1$ ), 4.2 and 4.3. Define  $\{\Psi_{l,p}\}$  as the coefficients matrices in the power series of  $(\mathbf{I}_r - \sum_{l=1}^p \mathbf{A}_{l,p} z^l)^{-1}$ , for  $|z| \leq 1$  with  $\Psi_{0,q} := \mathbf{I}_r$ . Similarly, define  $\{\tilde{\Psi}_{l,p}\}$  as the power series coefficients matrices of  $(\mathbf{I}_r - \sum_{l=1}^p \tilde{\mathbf{A}}_{l,p} z^l)^{-1}$ , for  $|z| \leq 1$  with  $\tilde{\Psi}_{0,q} := \mathbf{I}_r$ , and  $\{\hat{\Psi}_{l,p}\}$  as the power series coefficients matrices of  $(\mathbf{I}_r - \sum_{l=1}^p \hat{\mathbf{A}}_{l,p} z^l)^{-1}$ ,

for  $|z| \leq 1$  with  $\widehat{\Psi}_{0,q} := \mathbf{I}_r$ . Then, there exists  $p_3 \in \mathbb{N}$  such that for all  $p \geq p_3$  as in Lemma C.6,

$$\begin{aligned} \sum_{l=1}^{\infty} \left\| \widetilde{\Psi}_{l,p} - \Psi_{l,p} \right\|_F &= O_P \left( \frac{1}{p} \right) = o_P(1), \\ \sum_{l=1}^{\infty} \left\| \Psi_{l,p} - \Psi_l \right\|_F &= o(1), \\ \sum_{l=1}^{\infty} \left\| \widehat{\Psi}_{l,p} - \widetilde{\Psi}_{l,p} \right\|_F &= O_P \left( p^{3/2} \left\| \widehat{\mathbf{A}}_p - \widetilde{\mathbf{A}}_p \right\|_F \right) = o_P(1), \\ \sum_{l=1}^{\infty} \left\| \widehat{\Psi}_{l,p} - \Psi_{l,p} \right\|_F &= o_P(1), \end{aligned}$$

when  $N \rightarrow \infty$  and  $T \rightarrow \infty$ .

*Proof of Lemma C.7.* For large enough  $N, T$  and  $p > p_3$  as in Lemma C.6,  $\sum_{l=1}^{\infty} \left\| \widetilde{\Psi}_{l,p} - \Psi_{l,p} \right\|_F$  follows directly from Lemma C.6 as

$$\begin{aligned} \sum_{l=1}^{\infty} \left\| \widetilde{\Psi}_{l,p} - \Psi_{l,p} \right\|_F &\leq \frac{1}{p^2} \sum_{l=1}^{\infty} \left( 1 + \frac{1}{p} \right)^{-l} O_P(1) \\ &\leq \frac{1}{p^2} \frac{p}{1+p} (1+p) O_P(1) \\ &= O_P \left( \frac{1}{p} \right). \end{aligned}$$

The order of  $\sum_{l=1}^{\infty} \left\| \Psi_{l,p} - \Psi_l \right\|_F$  follows directly from Lemma C.5 (i) and (iv), as

$$\begin{aligned} \sum_{l=1}^{\infty} \left\| \Psi_{l,p} - \Psi_l \right\|_F &\leq \sum_{l=1}^{\infty} (1+l)^{\gamma} \left\| \Psi_{l,p} - \Psi_l \right\|_F \\ &\leq d \sum_{l=p+1}^{\infty} (1+l)^{\gamma} \left\| \mathbf{A}_l \right\|_F \\ &= o(1). \end{aligned}$$

To show  $\sum_{l=1}^{\infty} \left\| \widehat{\Psi}_{l,p} - \widetilde{\Psi}_{l,p} \right\|_F = o_P(1)$ , first notice that

$$\sum_{l=1}^{\infty} \left\| \widehat{\Psi}_{l,p} - \widetilde{\Psi}_{l,p} \right\|_F \leq \sum_{l=1}^{\infty} \sum_{u=1}^r \sum_{v=1}^r \left| \widehat{\Psi}_{l,p}^{(u,v)} - \widetilde{\Psi}_{l,p}^{(u,v)} \right|,$$

where  $\widehat{\Psi}_{l,p}^{(u,v)}$  and  $\widetilde{\Psi}_{l,p}^{(u,v)}$  are the  $(u, v)^{\text{th}}$  elements of the matrices  $\widehat{\Psi}_{l,p}$  and  $\widetilde{\Psi}_{l,p}$ , respectively. We then apply Cauchy's inequality for holomorphic functions on the  $(u, v)^{\text{th}}$  element of  $\widetilde{\Psi}_{l,p}$  and

$\Psi_{l,p}$ , that is

$$\begin{aligned}
\left| \widehat{\Psi}_{l,p}^{(u,v)} - \widetilde{\Psi}_{l,p}^{(u,v)} \right| &\leq \left(1 + \frac{1}{p}\right)^{-l} \max_{|z|=1+\frac{1}{p}} \left\| \widehat{\mathbf{A}}_p^{-1}(z) - \widetilde{\mathbf{A}}_p^{-1}(z) \right\|_F \\
&\leq \left(1 + \frac{1}{p}\right)^{-l} \left[ \max_{|z|=1+\frac{1}{p}} \frac{1}{|\det(\widehat{\mathbf{A}}_p(z))|} \left\| \widehat{\mathbf{A}}_p^{adj}(z) - \widetilde{\mathbf{A}}_p^{adj}(z) \right\|_F \right. \\
&\quad \left. + \max_{|z|=1+\frac{1}{p}} \left| \frac{1}{\det(\widehat{\mathbf{A}}_p(z))} - \frac{1}{\det(\widetilde{\mathbf{A}}_p(z))} \right| \left\| \widetilde{\mathbf{A}}_p^{adj}(z) \right\|_F \right] \\
&=: \left(1 + \frac{1}{p}\right)^{-l} \left[ \max_{|z|=1+\frac{1}{p}} \mathcal{K}_{1,z} + \max_{|z|=1+\frac{1}{p}} \mathcal{K}_{2,z} \right],
\end{aligned}$$

where we use  $\mathbf{A}^{adj}$  to denote the adjugate matrix of  $\mathbf{A}$ , and write the two terms above as  $\mathcal{K}_{1,z}$  and  $\mathcal{K}_{2,z}$ .

To study  $\mathcal{K}_{1,z}$ , with Assumption 4.2, Lemmas C.2 and C.4, we show that with sufficiently large  $N$  and  $T$ , we can choose  $p > p_3$  such that  $\left\| \widehat{\mathbf{A}}_p - \widetilde{\mathbf{A}}_p \right\|_F = o_P(1)$  and  $\sup_{|z| \leq 1+\frac{1}{p}} \left\| \widehat{\mathbf{A}}_p(z) - \widetilde{\mathbf{A}}_p(z) \right\|_F = o_P(1)$ . Furthermore, since determinants are continuous functions of the elements, it can be extended to  $\sup_{|z| \leq 1+\frac{1}{p}} \left| \det \widehat{\mathbf{A}}_p(z) - \det \widetilde{\mathbf{A}}_p(z) \right| \rightarrow 0$  in probability, with

$$\left| \det \left( \widetilde{\mathbf{A}}_p(z) \right) \right| \geq c \text{ and } \left| \det \left( \widehat{\mathbf{A}}_p(z) \right) \right| \geq c \text{ in probability, for } |z| \leq 1 + \frac{1}{p},$$

and for some  $c > 0$  as in Lemma C.5. Then, for  $p > p_3$  and any  $|z| = 1 + 1/p$  we can show that

$$\begin{aligned}
\mathcal{K}_{1,z} &\leq \frac{1}{c} \left\| \widehat{\mathbf{A}}_p^{adj}(z) - \widetilde{\mathbf{A}}_p^{adj}(z) \right\|_F \\
&\leq \frac{1}{c} \sum_{u=1}^r \sum_{v=1}^r \left| \widehat{\mathbf{A}}_p^{adj}(z)^{(u,v)} - \widetilde{\mathbf{A}}_p^{adj}(z)^{(u,v)} \right| \\
&\leq \frac{1}{c} \sum_{u=1}^r \sum_{v=1}^r \sup_{|z| \leq 1+\frac{1}{p}} \left| \det \widehat{\mathbf{A}}_p^{(-v,-u)}(z) - \det \widetilde{\mathbf{A}}_p^{(-v,-u)}(z) \right| \\
&\leq \frac{1}{c} \sum_{u=1}^r \sum_{v=1}^r \sup_{|z| \leq 1+\frac{1}{p}} r \left\| \widehat{\mathbf{A}}_p(z) - \widetilde{\mathbf{A}}_p(z) \right\|_F O_P(1) \\
&\leq \sup_{|z| \leq 1+\frac{1}{p}} \left\| \widehat{\mathbf{A}}_p(z) - \widetilde{\mathbf{A}}_p(z) \right\|_F,
\end{aligned}$$

where  $\widetilde{\mathbf{A}}_p^{(-v,-u)}(z)$  is a matrix generated by removing the  $v^{\text{th}}$  row and the  $u^{\text{th}}$  column of  $\widetilde{\mathbf{A}}_p(z)$ .

And for  $\sup_{|z| \leq 1 + \frac{1}{p}} \left\| \hat{\mathbf{A}}_p(z) - \tilde{\mathbf{A}}_p(z) \right\|_F$ , we have

$$\begin{aligned} \sup_{|z| \leq 1 + \frac{1}{p}} \left\| \hat{\mathbf{A}}_p(z) - \tilde{\mathbf{A}}_p(z) \right\|_F &\leq \sup_{|z| \leq 1 + \frac{1}{p}} \sum_{l=1}^p \left\| \hat{\mathbf{A}}_{l,p} - \tilde{\mathbf{A}}_{l,p} \right\|_F |Z|^l \\ &\leq \left(1 + \frac{1}{p}\right)^p \sum_{l=1}^p \left\| \hat{\mathbf{A}}_{l,p} - \tilde{\mathbf{A}}_{l,p} \right\|_F \\ &= O_P \left( \sqrt{p} \left\| \hat{\mathbf{A}}_p - \tilde{\mathbf{A}}_p \right\|_F \right). \end{aligned}$$

Hence we can conclude that for  $\mathcal{K}_{1,z}$ ,

$$\max_{|z| \leq 1 + \frac{1}{p}} \mathcal{K}_{1,z} = O_P \left( \sqrt{p} \left\| \hat{\mathbf{A}}_p - \tilde{\mathbf{A}}_p \right\|_F \right),$$

since the bound does not depend on  $z$ .

For  $\mathcal{K}_{2,z}$ , note that  $\max_{|z| \leq 1 + \frac{1}{p}} \left\| \mathbf{A}_p(z) \right\|_F \leq (1 + 1/p)^p \sum_{l=1}^p \left\| \mathbf{A}_{l,p} \right\|_F = O_P(1)$  by Lemma C.5, therefore,  $\max_{|z| \leq 1 + \frac{1}{p}} \left\| \tilde{\mathbf{A}}_p(z) \right\|_F = O_P(1)$  by Assumption 4.2. Similarly, for some constants  $c$ ,

$$\begin{aligned} \max_{|z| \leq 1 + \frac{1}{p}} \mathcal{K}_{2,z} &\leq \frac{1}{c^2} \max_{|z| \leq 1 + \frac{1}{p}} \left| \det \hat{\mathbf{A}}_p(z) - \det \tilde{\mathbf{A}}_p(z) \right| \left\| \tilde{\mathbf{A}}_p^{adj}(z) \right\|_F \\ &= O_P \left( \sqrt{p} \left\| \hat{\mathbf{A}}_p - \tilde{\mathbf{A}}_p \right\|_F \right). \end{aligned}$$

As a result,

$$\begin{aligned} \sum_{l=1}^{\infty} \left\| \hat{\Psi}_{l,p} - \tilde{\Psi}_{l,p} \right\|_F &\leq \sum_{l=1}^{\infty} \sum_{u=1}^r \sum_{v=1}^r \left| \hat{\Psi}_{l,p}^{(u,v)} - \tilde{\Psi}_{l,p}^{(u,v)} \right| \\ &= O_P \left( p^{3/2} \left\| \hat{\mathbf{A}}_p - \tilde{\mathbf{A}}_p \right\|_F \right). \end{aligned}$$

Then, we can conclude that

$$\begin{aligned} \sum_{l=1}^{\infty} \left\| \hat{\Psi}_{l,p} - \Psi_{l,p} \right\|_F &\leq \sum_{l=1}^{\infty} \left\| \tilde{\Psi}_{l,p} - \Psi_{l,p} \right\|_F + \sum_{l=1}^{\infty} \left\| \hat{\Psi}_{l,p} - \tilde{\Psi}_{l,p} \right\|_F \\ &= O_P \left( \frac{1}{p} \right) + O_P \left( p^{3/2} \left\| \hat{\mathbf{A}}_p - \tilde{\mathbf{A}}_p \right\|_F \right). \end{aligned}$$

□

**Lemma C.8.** Let  $\{f_t\}$  be factor processes defined under the assumptions of Lemma C.7. Write  $\mathbf{e}_t = \mathbf{f}_t - \sum_{l=1}^{\infty} \mathbf{A}_l \mathbf{f}_{t-l}$ ,  $\mathbf{e}_{t,p} = \mathbf{f}_t - \sum_{l=1}^p \mathbf{A}_{l,p} \mathbf{f}_{t-l}$ ,  $\tilde{\mathbf{e}}_{t,p} = \mathbf{f}_t - \sum_{l=1}^p \tilde{\mathbf{A}}_{l,p} \mathbf{f}_{t-l}$  and  $\hat{\mathbf{e}}_{t,p} = \hat{\mathbf{f}}_t - \sum_{l=1}^p \hat{\mathbf{A}}_{l,p} \hat{\mathbf{f}}_{t-l}$ .

Furthermore, define the corresponding covariance  $\tilde{\Sigma}_{e,p} = \mathbb{E}^*(\tilde{\mathbf{e}}_{t,p} - \tilde{\mathbf{e}}_{T,p})(\tilde{\mathbf{e}}_{t,p} - \tilde{\mathbf{e}}_{T,p})^\top$  with  $\tilde{\mathbf{e}}_{T,p} = \frac{1}{T-p} \sum_{t=p+1}^T \tilde{\mathbf{e}}_{t,p}$ , and  $\hat{\Sigma}_{e,p} = \mathbb{E}^*(\hat{\mathbf{e}}_{t,p} - \hat{\mathbf{e}}_{T,p})(\hat{\mathbf{e}}_{t,p} - \hat{\mathbf{e}}_{T,p})^\top$  with  $\hat{\mathbf{e}}_{T,p} = \frac{1}{T-p} \sum_{t=p+1}^T \hat{\mathbf{e}}_{t,p}$ , where  $\mathbb{E}^*$  is the expectation defined on the measure of assigning probability  $\frac{1}{T-p}$  to each observation.

If we additionally assume that the empirical distribution of  $\{\mathbf{e}_t\}$  converges weakly to the distribution function of  $\mathcal{L}(\mathbf{e}_t)$ , then, there exists  $p_3 \in \mathbb{N}$  such that for all  $p \geq p_3$  as in Lemma C.6,

$$\begin{aligned}\|\tilde{\Sigma}_{e,p} - \Sigma_{e,p}\|_F &= o_P(1), \\ \|\Sigma_{e,p} - \Sigma_e\|_F &= o(1), \\ \|\hat{\Sigma}_{e,p} - \tilde{\Sigma}_{e,p}\|_F &= O_P\left(p^{3/2} \|\hat{\mathbf{A}}_p - \tilde{\mathbf{A}}_p\|_F\right) = o_P(1), \\ \|\hat{\Sigma}_{e,p} - \Sigma_{e,p}\|_F &= o_P(1),\end{aligned}$$

when  $N \rightarrow \infty$  and  $T \rightarrow \infty$ .

*Proof of Lemma C.8.* To show  $\|\tilde{\Sigma}_{e,p} - \Sigma_{e,p}\|_F \rightarrow 0$  in probability, first note that by definition,

$$\begin{aligned}\|\tilde{\Sigma}_{e,p} - \Sigma_{e,p}\|_F &= \left\| \frac{1}{T-p} \sum_{t=p+1}^T (\tilde{\mathbf{e}}_{t,p} \tilde{\mathbf{e}}_{t,p}^\top - \mathbf{e}_{t,p} \mathbf{e}_{t,p}^\top) \right\|_F \\ &\quad + \left\| \frac{1}{T-p} \sum_{t=p+1}^T \mathbf{e}_{t,p} \mathbf{e}_{t,p}^\top - \mathbb{E}(\mathbf{e}_{t,p} \mathbf{e}_{t,p}^\top) \right\|_F \\ &\quad + \|\tilde{\mathbf{e}}_{T,p} \tilde{\mathbf{e}}_{T,p}^\top\|_F \\ &=: \mathcal{E}_1 + \mathcal{E}_2 + \mathcal{E}_3,\end{aligned}$$

with straightforward notations for  $\mathcal{E}_1$ ,  $\mathcal{E}_2$  and  $\mathcal{E}_3$ . Next, we show that the three terms above converge to zero in probability. For  $\mathcal{E}_1$ , we know that by triangular inequality,

$$\begin{aligned}\mathcal{E}_1 &\leq \left\| \frac{1}{T-p} \sum_{t=p+1}^T (\tilde{\mathbf{e}}_{t,p} - \mathbf{e}_{t,p}) \tilde{\mathbf{e}}_{t,p}^\top \right\|_F + \left\| \frac{1}{T-p} \sum_{t=p+1}^T \mathbf{e}_{t,p} (\tilde{\mathbf{e}}_{t,p} - \mathbf{e}_{t,p})^\top \right\|_F \\ &=: \mathcal{E}_{1,1} + \mathcal{E}_{1,2},\end{aligned}$$

with obvious notations for  $\mathcal{E}_{1,1}$  and  $\mathcal{E}_{1,2}$ . It is then sufficient to show  $\mathcal{E}_{1,1} \rightarrow 0$  in probability since

$\mathcal{E}_{1,2}$  can be dealt with in a similar way. We can now bound  $\mathcal{E}_{1,1}$  by

$$\begin{aligned}\mathcal{E}_{1,1} &\leq \left\| \frac{1}{T-p} \sum_{t=p+1}^T \sum_{l=1}^p (\tilde{\mathbf{A}}_{l,p} - \mathbf{A}_{l,p}) \mathbf{f}_{t-l} \tilde{\mathbf{e}}_{t,p}^\top \right\|_F \\ &\quad + \left\| \frac{1}{T-p} \sum_{t=p+1}^T \sum_{l=1}^p (\mathbf{A}_{l,p} - \mathbf{A}_l) \mathbf{f}_{t-l} \tilde{\mathbf{e}}_{t,p}^\top \right\|_F \\ &\quad + \left\| \frac{1}{T-p} \sum_{t=p+1}^T \sum_{l=p+1}^{\infty} \mathbf{A}_l \mathbf{f}_{t-l} \tilde{\mathbf{e}}_{t,p}^\top \right\|_F.\end{aligned}$$

Since both  $\{\mathbf{f}_t\}$  and  $\{\tilde{\mathbf{e}}_{t,p}\}$  are  $r \times 1$  vectors, by Assumption 4.2 and Lemma C.5, we have

$$\mathcal{E}_{1,1} = O_P \left( \left\| \sum_{l=1}^p (\tilde{\mathbf{A}}_{l,p} - \mathbf{A}_{l,p}) \right\|_F + \sum_{l=p+1}^{\infty} (1+l) \|\mathbf{A}_l\|_F \right),$$

which tends to zero in probability.

$\mathcal{E}_2 \rightarrow 0$  in probability can be shown similarly, since  $\{\mathbf{f}_t\}$  is stationary. For  $\mathcal{E}_3$ , first write that

$$\begin{aligned}\mathcal{E}_3 &= \left\| \tilde{\mathbf{e}}_{T,p} \tilde{\mathbf{e}}_{T,p}^\top \right\|_F \\ &\leq \left\| (\tilde{\mathbf{e}}_{T,p} - \bar{\mathbf{e}}_{T,p}) (\tilde{\mathbf{e}}_{T,p} - \bar{\mathbf{e}}_{T,p})^\top \right\|_F + 2 \left\| (\tilde{\mathbf{e}}_{T,p} - \bar{\mathbf{e}}_{T,p}) \bar{\mathbf{e}}_{T,p}^\top \right\|_F + \left\| \bar{\mathbf{e}}_{T,p} \bar{\mathbf{e}}_{T,p}^\top \right\|_F,\end{aligned}$$

where  $\|\bar{\mathbf{e}}_{T,p}\| = O_P((T-p)^{-1/2})$ . Hence it is sufficient to consider  $\|\tilde{\mathbf{e}}_{T,p} - \bar{\mathbf{e}}_{T,p}\|$  as

$$\begin{aligned}\|\tilde{\mathbf{e}}_{T,p} - \bar{\mathbf{e}}_{T,p}\| &= \left\| \frac{1}{T-p} \sum_{t=p+1}^T (\tilde{\mathbf{e}}_{t,p} - \mathbf{e}_{t,p}) \right\| \\ &= \left\| \frac{1}{T-p} \sum_{t=p+1}^T \left( \sum_{l=1}^p \tilde{\mathbf{A}}_{l,p} \mathbf{f}_{t-l} - \sum_{l=1}^{\infty} \mathbf{A}_l \mathbf{f}_{t-l} \right) \right\| \\ &\leq \left\| \frac{1}{T-p} \sum_{t=p+1}^T \sum_{l=1}^p (\tilde{\mathbf{A}}_{l,p} - \mathbf{A}_{l,p}) \mathbf{f}_{t-l} \right\| \\ &\quad + \left\| \frac{1}{T-p} \sum_{t=p+1}^T \sum_{l=1}^p (\mathbf{A}_{l,p} - \mathbf{A}_l) \mathbf{f}_{t-l} \right\| + \left\| \frac{1}{T-p} \sum_{t=p+1}^T \sum_{l=p+1}^{\infty} \mathbf{A}_l \mathbf{f}_{t-l} \right\| \\ &= O_P \left( \left\| \sum_{l=1}^p (\tilde{\mathbf{A}}_{l,p} - \mathbf{A}_{l,p}) \right\|_F \right) + O_P \left( \sum_{l=p+1}^{\infty} (1+l) \|\mathbf{A}_l\|_F \right) \xrightarrow{p} 0,\end{aligned}$$

where the last line follows from Assumption 4.2 and Lemma C.5, and we use the same arguments for  $\mathcal{E}_{1,1}$  as above. Therefore, we can conclude that  $\|\tilde{\boldsymbol{\Sigma}}_{e,p} - \boldsymbol{\Sigma}_{e,p}\|_F \rightarrow 0$  in probability.

To see  $\|\Sigma_{e,p} - \Sigma_e\|_F \rightarrow 0$ , note that

$$\begin{aligned}\|\Sigma_{e,p} - \Sigma_e\|_F &= \left\| \mathbb{E} \left( \mathbf{e}_{t,p} \mathbf{e}_{t,p}^\top - \mathbf{e}_t \mathbf{e}_t^\top \right) \right\|_F \\ &\leq \left\| \mathbb{E} \left\{ (\mathbf{e}_{t,p} - \mathbf{e}_t) \mathbf{e}_{t,p}^\top \right\} \right\|_F + \left\| \mathbb{E} \left\{ \mathbf{e}_{t,p} (\mathbf{e}_{t,p} - \mathbf{e}_t)^\top \right\} \right\|_F.\end{aligned}$$

Hence it suffices to show  $\left\| \mathbb{E} \left\{ (\mathbf{e}_{t,p} - \mathbf{e}_t) \mathbf{e}_{t,p}^\top \right\} \right\|_F \rightarrow 0$ . For this, by triangular inequality, we have

$$\begin{aligned}\left\| \mathbb{E} \left\{ (\mathbf{e}_{t,p} - \mathbf{e}_t) \mathbf{e}_{t,p}^\top \right\} \right\|_F &\leq \left\| \mathbb{E} \sum_{l=1}^p (\mathbf{A}_{l,p} - \mathbf{A}_l) \mathbf{f}_{t-l} \mathbf{e}_{t,p}^\top \right\|_F + \left\| \mathbb{E} \sum_{l=p+1}^{\infty} \mathbf{A}_l \mathbf{f}_{t-l} \mathbf{e}_{t,p}^\top \right\|_F \\ &= O \left( \sum_{l=1}^p \|\mathbf{A}_{l,p} - \mathbf{A}_l\|_F \right) + O \left( \sum_{l=p+1}^{\infty} \|\mathbf{A}_l\|_F \right) \rightarrow 0,\end{aligned}$$

where we stress the fact that  $\|\mathbf{f}_t\| \asymp \|\mathbf{e}_{t,p}\| \asymp 1$  and use the results in Lemma C.5.

With similar arguments, we can show that  $\|\widehat{\Sigma}_{e,p} - \widetilde{\Sigma}_{e,p}\|_F \rightarrow 0$  in probability. Firstly, notice that  $(\widehat{\Sigma}_{e,p} - \widetilde{\Sigma}_{e,p})$  can be expressed as

$$\begin{aligned}\widehat{\Sigma}_{e,p} - \widetilde{\Sigma}_{e,p} &= \frac{1}{T-p} \sum_{t=p+1}^T \left[ (\widehat{\mathbf{e}}_{t,p} - \widetilde{\mathbf{e}}_{T,p}) (\widehat{\mathbf{e}}_{t,p} - \widetilde{\mathbf{e}}_{T,p})^\top - (\widetilde{\mathbf{e}}_{t,p} - \widetilde{\mathbf{e}}_{T,p}) (\widetilde{\mathbf{e}}_{t,p} - \widetilde{\mathbf{e}}_{T,p})^\top \right] \\ &= \frac{1}{T-p} \sum_{t=p+1}^T \left[ (\widehat{\mathbf{e}}_{t,p} - \widetilde{\mathbf{e}}_{T,p}) - (\widetilde{\mathbf{e}}_{t,p} - \widetilde{\mathbf{e}}_{T,p}) \right] (\widehat{\mathbf{e}}_{t,p} - \widetilde{\mathbf{e}}_{t,p})^\top \\ &\quad - \frac{1}{T-p} \sum_{t=p+1}^T \left[ (\widehat{\mathbf{e}}_{t,p} - \widetilde{\mathbf{e}}_{T,p}) - (\widetilde{\mathbf{e}}_{t,p} - \widetilde{\mathbf{e}}_{T,p}) \right] (\widetilde{\mathbf{e}}_{T,p} - \widetilde{\mathbf{e}}_{t,p})^\top \\ &\quad + \frac{1}{T-p} \sum_{t=p+1}^T \left[ (\widehat{\mathbf{e}}_{t,p} - \widetilde{\mathbf{e}}_{T,p}) (\widetilde{\mathbf{e}}_{t,p} - \widetilde{\mathbf{e}}_{T,p})^\top \right] \\ &\quad + \frac{1}{T-p} \sum_{t=p+1}^T \left[ (\widetilde{\mathbf{e}}_{t,p} - \widetilde{\mathbf{e}}_{T,p}) (\widehat{\mathbf{e}}_{t,p} - \widetilde{\mathbf{e}}_{T,p})^\top \right].\end{aligned}$$

Recall that  $\widetilde{\mathbf{e}}_{T,p} = \frac{1}{T-p} \sum_{t=p+1}^T \widetilde{\mathbf{e}}_{t,p}$  and  $\widetilde{\mathbf{e}}_{T,p} = \frac{1}{T-p} \sum_{t=p+1}^T \widehat{\mathbf{e}}_{t,p}$ , therefore, by triangular inequality, it is sufficient to study the leading term  $\frac{1}{T-p} \sum_{t=p+1}^T \left[ (\widehat{\mathbf{e}}_{t,p} - \widetilde{\mathbf{e}}_{t,p}) - (\widetilde{\mathbf{e}}_{t,p} - \widetilde{\mathbf{e}}_{t,p}) \right] (\widehat{\mathbf{e}}_{t,p} - \widetilde{\mathbf{e}}_{t,p})^\top$ . For this, it is sufficient to consider the order of  $\left\| \frac{1}{T-p} \sum_{t=p+1}^T (\widehat{\mathbf{e}}_{t,p} - \widetilde{\mathbf{e}}_{t,p}) (\widehat{\mathbf{e}}_{t,p} - \widetilde{\mathbf{e}}_{t,p})^\top \right\|_F$ . We then



have the bound

$$\begin{aligned}
\frac{1}{T-p} \sum_{t=p+1}^T \|\widehat{e}_{t,p} - \widetilde{e}_{t,p}\|^2 &\leq 3 \sum_{l=1}^p \left\| \widehat{\mathbf{A}}_{l,p} - \widetilde{\mathbf{A}}_{l,p} \right\|_F^2 \frac{1}{T-p} \sum_{t=p+1}^T \left\| \widehat{\mathbf{f}}_{t-l} \right\|^2 \\
&\quad + \frac{3}{T-p} \sum_{t=p+1}^T \left\| \widehat{\mathbf{f}}_t - \mathbf{f}_t \right\|^2 + 3 \sum_{l=1}^p \left\| \widetilde{\mathbf{A}}_{l,p} \right\|_F^2 \frac{1}{T-p} \sum_{t=p+1}^T \left\| \widehat{\mathbf{f}}_{t-l} - \mathbf{f}_{t-l} \right\|^2 \\
&= O_P \left( \left\| \widehat{\mathbf{A}}_p - \widetilde{\mathbf{A}}_p \right\|_F^2 \right) + O_P \left( p \left\| \widehat{\mathbf{f}}_t - \mathbf{f}_t \right\|^2 \right),
\end{aligned}$$

which converges to 0 in probability by the results of Lemmas C.3 and C.4. Hence we can conclude that  $\left\| \widehat{\boldsymbol{\Sigma}}_{e,p} - \widetilde{\boldsymbol{\Sigma}}_{e,p} \right\|_F \rightarrow 0$  in probability.

Lastly,  $\left\| \widehat{\boldsymbol{\Sigma}}_{e,p} - \boldsymbol{\Sigma}_{e,p} \right\|_F = o_P(1)$  follows directly from  $\left\| \widehat{\boldsymbol{\Sigma}}_{e,p} - \widetilde{\boldsymbol{\Sigma}}_{e,p} \right\|_F = o_P(1)$ ,  $\left\| \widetilde{\boldsymbol{\Sigma}}_{e,p} - \boldsymbol{\Sigma}_{e,p} \right\|_F = o_P(1)$ , and the triangular inequality.  $\square$
